# Supplementary material for: Optimal Estimation of Large-Dimensional Nonlinear Factor Models
Source: arXiv:2311.07243 source file (2026-09-30)
Supplement: Supplementary file 1 [file supp.tex]

\documentclass[12pt]{article}
\pdfoutput=1
\usepackage{filecontents}
\usepackage{amsfonts,amssymb,amsmath,amsthm,dsfont,graphicx,hyperref,mathrsfs,euscript,enumitem,framed, bm}
\usepackage[title, titletoc]{appendix}
\usepackage[top=1in,bottom=1in,left=1in,right=1in]{geometry} % the layout package
\usepackage[onehalfspacing]{setspace}
\usepackage{ifthen,caption,subcaption,lscape}
\hypersetup{pdfborder = {0 0 0},colorlinks=true,linkcolor=blue,urlcolor=blue,citecolor=blue}
\usepackage{chngcntr} 
\usepackage{natbib}
\usepackage{longtable}
\usepackage{placeins}
\usepackage{xr-hyper}
\externaldocument{file} 

\newtheorem{thm}{Theorem}

\newtheorem{lem}{Lemma}
\newtheorem{assumption}{Assumption}

\theoremstyle{definition}

%%% REMARK
\theoremstyle{definition}
\newtheorem{remark_tmp}{Remark}[section]
\newenvironment{remark}
{ \begin{remark_tmp} 	}
	{ 
		%\renewcommand{\bqedsymbol}{$\bm{\ell}acksquare$}
		%\medskip\bqed 
		\medskip\hfill{\LARGE$\lrcorner$}
	\end{remark_tmp} 
}

\newtheorem{exmp}{Example}[section]

\allowdisplaybreaks[1]

%New operators: trace, argmin, argmax, etc

\DeclareMathOperator*{\tr}{Tr}

\DeclareMathOperator*{\diag}{diag}

%independence

% % % % % % % % % % % % % % Some Notations % % % % % % % % % % % % % %
\renewcommand{\P}{\mathbb{P}}
\newcommand{\E}{\mathbb{E}}

\newcommand{\I}{\mathds{1}}

% % % % % % % % % Special subscript  % % % % % % % % %%
\newcommand{\subi}{\langle i \rangle}
\newcommand{\gr}[1]{\cdot\mathcal{C}_{#1}}

% % % % % % % % % % % % % % Bold letters % % % % % % % % % % % % % %
\newcommand{\bA}{\bm{A}}
\newcommand{\bH}{\bm{H}}

\newcommand{\bB}{\bm{B}}

\newcommand{\bF}{\bm{F}}
\newcommand{\bG}{\bm{G}}
\newcommand{\bff}{\mathbf{f}}
\newcommand{\bI}{\bm{I}}

\newcommand{\bM}{\bm{M}}

\newcommand{\bP}{\bm{P}}

\newcommand{\bR}{\bm{R}}

\newcommand{\bU}{\bm{U}}
\newcommand{\bT}{\bm{T}}

\newcommand{\bW}{\bm{W}}
\newcommand{\bX}{\bm{X}}

\newcommand{\ba}{\bm{a}}

\newcommand{\bc}{\bm{c}}
\newcommand{\bg}{\bm{g}}
\newcommand{\be}{\bm{e}}

\newcommand{\bh}{\bm{h}}

\newcommand{\bu}{\bm{u}}
\newcommand{\bv}{\bm{v}}
\newcommand{\bx}{\bm{x}}

\newcommand{\bw}{\bm{w}}
\newcommand{\bz}{\bm{z}}

\newcommand{\balpha}{\boldsymbol{\alpha}}

\newcommand{\bbeta}{\boldsymbol{\beta}}

\newcommand{\bXi}{\boldsymbol{\Xi}}
\newcommand{\bvth}{\boldsymbol{\vartheta}}

\newcommand{\bSigma}{\boldsymbol{\Sigma}}
\newcommand{\bUpsilon}{\boldsymbol{\Upsilon}}

\newcommand{\blambda}{\boldsymbol{\lambda}}
\newcommand{\bLambda}{\boldsymbol{\Lambda}}
\newcommand{\bmeta}{\boldsymbol{\eta}}
\newcommand{\bvrho}{\boldsymbol{\varrho}}

\newcommand{\bOmega}{\boldsymbol{\Omega}}

\newcommand{\lvarsig}{\underline{\varsigma}}
\newcommand{\uvarsig}{\bar{\varsigma}}

\newcommand{\ttd}{\mathsf{d}}

\setlength{\parindent}{1em}

\setlength{\bibsep}{0.0pt}

 % I just don't like typing out varepsilon

\setenumerate[1]{label=\bf(\alph*)}

%%%%%%%%%%%%%%%%%%%%%%%%%%%%%

%\renewcommand{\theprop}{SA\arabic{prop}}\setcounter{prop}{0}

%\numberwithin{assumption}{section}
\numberwithin{equation}{section}
\numberwithin{thm}{section}
\numberwithin{lem}{section}
\numberwithin{assumption}{section}
\numberwithin{coro}{thm}

%\renewcommand{\thepart}{SA-\arabic{part}}
%\setcounter{part}{-1}
%\counterwithin{section}{part}
%\renewcommand*\thesection{\thepart.\arabic{section}}
%%%%%%%%%%%%%%%%%%%%%%%%%%%%%
\newcommand{\forloop}[5][1]{\setcounter{#2}{#3}\ifthenelse{#4}{#5\addtocounter{#2}{#1}\forloop[#1]{#2}{\value{#2}}{#4}{#5}}{}}

%%%%%%%%%%%%%%%%%%%
\usepackage{tocloft}
\addtolength{\cftsecnumwidth}{25pt}
\addtolength{\cftsubsecnumwidth}{25pt}
\addtolength{\cftsubsubsecnumwidth}{25pt}
%%%%%%%%%%%%%%%%%%%

\begin{document}

% % % % % % % % % % % % % % Title Page % % % % % % % % % % % % % %
\title{\vspace{-0.25in}\Large Optimal Estimation of Large-Dimensional Nonlinear Factor Models\\
	\medskip
	Supplemental Appendix
\bigskip }
\author{
	Yingjie Feng\thanks{School of Economics and Management, Tsinghua University.}}
\maketitle

\vspace{1em}

\begin{abstract}
This supplement gives omitted theoretical proofs of the results discussed in the main paper, and additional technical and numerical results, which may be of independent interest. Section \ref{SA-sec: main results} presents the formal theory for the more general covariates-adjusted nonlinear factor model.
Section \ref{SA-sec: discussion of conditions} gives some further discussion about the conditions imposed in the main paper. 
Section \ref{SA-sec: proofs} gives all omitted proofs for the main paper as well as proofs  for this supplement. Section \ref{SA-sec: simulation} gives additional simulation results.  
\end{abstract}

\thispagestyle{empty}

\newpage\tableofcontents

\thispagestyle{empty}
\clearpage

%\doublespacing
\setcounter{page}{1}
\pagestyle{plain}

% % % % % % % % % % % % % % Beginning of the Document % % % % % % % % % % % % % %

%SUMMARIZE and COMPARE RESULTS

\medskip
\section{Notation}

We introduce the notation used in this supplement below.

\textbf{Latent functions.} For a generic sequence of functions $\{h_t(\cdot):1\leq t\leq M\}$ defined on a compact support, let $\nabla^{\ell}\bh_t(\cdot)$ be a vector of $\ell$th-order partial derivatives of $h_t(\cdot)$, and define $\mathscr{D}^{[\kappa]}\bh_t(\cdot)=(\nabla^{0}\bh_t(\cdot)', \cdots, \nabla^{\kappa}\bh_t(\cdot)')'$, i.e., a column vector that stores all partial derivatives of $h_t(\cdot)$ up to order $\kappa\geq 0$. The derivatives on the boundary are understood as limits with the arguments ranging within the support.
When $\ell=1$, $\nabla\bh_t(\cdot):=\nabla^1\bh_t(\cdot)$ is the gradient vector, and the Jacobian matrix is 
$\nabla\bh(\cdot):=(\nabla\bh_1(\cdot), \cdots, \nabla\bh_{M}(\cdot))'$.

\textbf{Matrices.}
Several matrix norms are used throughout the paper. For a vector $\bv\in\mathbb{R}^{\ttd}$, $\|\bv\|=\sqrt{\bv'\bv}$ denotes its Euclidean norm. For an $m\times n$ matrix $\bA$, the Frobenius matrix norm is denoted by $\|\bA\|_{\tt F}=\sqrt{\tr(\bA\bA')}$,  
the $L^2$-operator norm by $\|\bA\|=s_1(\bA)$, and the entrywise sup-norm by $\|\bA\|_{\max}=\max_{1\leq i\leq m, 1\leq j\leq n}|a_{ij}|$, where $s_l(A)$ denotes the $l$th largest singular value of $\bA$.  To be more explicit, we write $s_{\max}(\bA):=s_1(\bA)$ and $s_{\min}(\bA):=s_{\min\{m,n\}}(\bA)$.  
Also, we use $\bA_{i\cdot}$ to denote the $i$th row and $\bA_{\cdot j}$ the $j$th column of $\bA$. More generally, for $\mathcal{C}\subseteq\{1,\cdots,n\}$ and $\mathcal{R}\subseteq\{1,\cdots, m\}$,  $\bA_{\cdot\mathcal{C}}$ denotes the submatrix of $\bA$ with column indices in $\mathcal{C}$, and $\bA_{\mathcal{R}\cdot}$ is the submatrix of $\bA$ with row indices in $\mathcal{R}$.

\textbf{Asymptotics.}
For sequences of numbers or random variables, $a_n\lesssim b_n$ denotes that $\limsup_n|a_n/b_n|$ is finite, and $a_n\lesssim_\P b_n$ or $a_n=O_\P(b_n)$ denotes  $\limsup_{\varepsilon\rightarrow\infty}\limsup_n\P[|a_n/b_n|\geq\varepsilon]=0$. $a_n=o(b_n)$ implies $a_n/b_n\rightarrow 0$, and $a_n=o_\P(b_n)$ implies $a_n/b_n\rightarrow_\P 0$, where $\rightarrow_\P$ denotes convergence in probability. $a_n\asymp b_n$ implies that $a_n\lesssim b_n$ and $b_n\lesssim a_n$, and $a_n\asymp_\P b_n$ implies $a_n\lesssim_\P b_n$ and $b_n\lesssim_\P a_n$.  For a sequence of random quantities \{$a_{n,i}:1\leq i\leq n\}$ indexed by $i$, $a_{n,i}$ is said to be $O_\P(b_n)$ (or $o_\P(b_n)$) uniformly over $1\leq i\leq n$, if $\max_{1\leq i\leq n}|a_{n,i}|=O_\P(b_n)$ (or $\max_{1\leq i\leq n}|a_{n,i}|=o_\P(b_n)$). %For two random variables $X$ and $Y$, $X=_d Y$ implies that they have the same probability distribution.
In addition, ``w.p.a. 1'' means ``with probability approaching one''.

\textbf{Others.}
For two numbers $a$ and $b$, $a\vee b=\max\{a,b\}$ and $a\wedge b=\min\{a,b\}$. For a finite set $\mathcal{S}$, $|\mathcal{S}|$ denotes its cardinality. $[m]$ denotes the set $\{1, \cdots, m\}$ for a positive integer $m$.
Let $\widehat{\blambda}_{j_k(i)}$ and $\blambda_{j_k(i)}$ be the local factor loadings in $\widehat{\bLambda}_{\subi}$ and $\bLambda_{\subi}$ respectively corresponding to the $j_k(i)$th unit.

%%%%%%%%%%%%%%%%%%%%%%%%%%%%%%%%%%%%%%%%%%%%%%%%%%%%%%%%%%%%%%%%%%%%%%%%%%%%%%%%%%%%%%%%%%%%%%
\section{Covariates-Adjusted Nonlinear Factor Model} \label{SA-sec: main results}

In this section we provide formal analysis of the generalized nonlinear factor model described in Section \ref{subsec: extensions}:
\begin{equation}\label{SA-eq: general model}
\bx_i=\bW_i\bvth+\bmeta(\balpha_i)+\bu_i, \quad \E[\bu_i|\mathscr{F}, \{\bW_i\}_{i=1}^n]=\bm{0}
\end{equation}
where $\bW_i=(\bw_{i,1}, \cdots, \bw_{i,q})$ is a $p\times q$ matrix of additional covariates, where $\bw_{i,\ell}=(w_{i1,\ell}, \cdots, w_{ip,\ell})'$ for each $\ell=1, \cdots, q$.

\subsection{Assumptions}

The following analysis is based on the main estimation procedure described in Section \ref{subsec: extensions} of the main paper. 
The first assumption concerns the structure of the high-rank covariates in Equation \eqref{SA-eq: general model}.

\begin{assumption}[High-Rank Covariates]
	\label{SA-Assumption: high-rank covariates}
	For $\ell=1, \ldots, q$, each $\bw_{i,\ell}$ satisfies that
	\[
	w_{it,\ell}=\hbar_{t,\ell}(\bvrho_{i,\ell})+e_{it,\ell}, \quad 
	\E[e_{it,\ell}|\mathcal{F}_\ell]=0,
	\]
	where $\{\bvrho_{i,\ell}\in\mathbb{R}^{r_{\ell}}:1\leq i\leq n\}$ is i.i.d. and  $\mathcal{F}_\ell$ is the $\sigma$-field generated by $\{\bvrho_{i,\ell}:1\leq i\leq n\}$ and $\{\hbar_{t,\ell}(\cdot):1\leq t\leq p,1\leq \ell\leq q\}$.
	Moreover, for some constant $c_{\min}>0$,
	$$s_{\min}\Big(\frac{1}{n|\mathcal{R}^\ddagger|}\sum_{i=1}^{n}\sum_{t\in\mathcal{R}^\ddagger}
	\be_{it}\be_{it}'\Big)\geq c_{\min} \quad \text{w.p.a. } 1,$$
	where $\be_{it}=(e_{it,1}, \cdots, e_{it,q})'$.
\end{assumption}

The condition above is akin to that commonly used in partially linear regression. It ensures that $\bw_{i,\ell}$'s are truly ``high-rank'': after partialling out the ``low-rank'' signals (factor components), these covariates are still non-degenerate, thus achieving identifiability of $\bvth$.
Also note that Assumption \ref{SA-Assumption: high-rank covariates} is general in the sense that the latent variables and latent functions associated with each $\bw_{i,\ell}$ could be different across $\ell$. To ease notation, introduce a $\sigma$-field $\mathcal{F}=\cup_{\ell=0}^{q}\mathcal{F}_\ell$ where $\mathcal{F}_0$ denotes the $\sigma$-field generated by $\{\balpha_i:1\leq i\leq n\}$. Let $\bar{r}$ be the number of \textit{distinct} variables among $\balpha_i,\bvrho_{i,1},\cdots, \bvrho_{i,q}$.

We impose some standard regularity conditions on the latent variables, latent functions and idiosyncratic errors, which are analogous 
to Assumption \ref{Assumption: Regularities} in the main paper.
\begin{assumption}[Regularities]
	\label{SA-Assumption: regularities}\leavevmode
	Let $\bar{m}\geq 2$ and $\nu>0$ be some constants.
	\begin{enumerate}[label=(\alph*)]
		\item For all $t\in [p]$, $\hbar_{t,\ell}(\cdot)$ and $\eta_t(\cdot)$ are $\bar{m}$-times continuously differentiable with all partial derivatives of order no greater than $\bar{m}$ bounded by a universal constant;
		
		\item $\{\balpha_i: 1\leq i\leq n\}$ and 
		$\{\bvrho_{i,\ell}: 1\leq i\leq n\}$ for each $\ell\in[q]$ have compact convex supports with densities bounded and bounded away from zero;
		
		\item Conditional on $\mathcal{F}$, $\{(u_{it}, \be_{it}):1\leq i\leq n,1\leq t\leq p\}$ is independent over $i$ and across $t$ with zero means, and 
		$\max_{1\leq i\leq n,1\leq t\leq p}\E[|u_{it}|^{2+\nu}|\mathcal{F}]<\infty$ and 
		$\max_{1\leq i\leq n,1\leq t\leq p}\E[|e_{it}|^{2+\nu}|\mathcal{F}]<\infty$ a.s. on $\mathcal{F}$;
	\end{enumerate}
\end{assumption}

Next, we impose conditions for indirect matching that is analogous to Assumption \ref{Assumption: Matching}.
To ease our exposition, for $\ell\in [q]$, we define the $p\times n$ matrices
$\bH$, $\bar{\bH}_{\lceil\ell\rfloor}$, $\bar{\bar{\bH}}$, $\bW_{\lceil \ell\rfloor}$ and $\tilde\bX$ whose $(t,i)$th elements are respectively given by
\begin{align*}
&H_{it}=\eta_t(\balpha_i),\quad
\bar{H}_{it, \lceil\ell\rfloor}=\hbar_{t,\ell}(\bvrho_{i,\ell}),\quad
\bar{\bar{H}}_{it}=\eta_t(\balpha_i)+\sum_{\ell=1}^{q}\hbar_{t,\ell}(\bvrho_{i,\ell})\vartheta_\ell, \\
&W_{it,\lceil\ell\rfloor}=w_{it,\ell},\quad \tilde{X}_{it}=\eta_t(\balpha_i)+u_{it}+\bW_i(\bvth-\widehat{\bvth}).
\end{align*}
As in the main paper, we use superscripts $\dagger$, $\ddagger$ and $\wr$ to 
denote the subset of features that belong to $\mathcal{R}^\dagger$, $\mathcal{R}^\ddagger$ and $\mathcal{R}^\wr$ respectively. 
For example, $\bH^{\dagger}$, $\bH^{\ddagger}$ and $\bH^{\wr}$ are submatrices of $\bH$ with row indices in $\mathcal{R}^\dagger$, $\mathcal{R}^\ddagger$ and $\mathcal{R}^\wr$ respectively.

\begin{assumption}[Indirect Matching] 
	\label{SA-Assumption: indirect matching}\leavevmode
		For some fixed positive constants $\rho_0$, $\lvarsig$, $\uvarsig$ and some positive sequence $a_{n}=o(1)$, the following conditions hold: 
		\[
		\begin{split}
		&\underset{1\leq i,j\leq n}{\max}\;|\rho(\bW_{\cdot i, \lceil\ell\rfloor}^\dagger, \bW_{\cdot j, \lceil\ell\rfloor}^\dagger)-
		\rho(\bar{\bH}_{\cdot i, \lceil\ell\rfloor}^\dagger, \bar\bH_{\cdot j, \lceil\ell\rfloor}^\dagger) 
		-\rho_0|\lesssim_\P a_{n}, \quad \ell\in[q],\\
		&\underset{1\leq i,j\leq n}{\max}\;|\rho(\bX_{\cdot i}^\dagger, \bX_{\cdot j}^\dagger)-
		\rho(\bar{\bar{\bH}}_{\cdot i}^\dagger, \bar{\bar{\bH}}_{\cdot j}^\dagger)
		-\rho_0|\lesssim_\P a_{n},\\
		&\underset{1\leq i,j\leq n}{\max}\;|\rho(\tilde\bX_{\cdot i}^\ddagger, \tilde\bX_{\cdot j}^\ddagger)-
		\rho(\bH_{\cdot i}^\ddagger, \bH_{\cdot j}^\ddagger)
		-\rho_0|\lesssim_\P a_{n},
		\end{split}
		\]
		and
		for each $\bM=\bH^{\ddagger}, \bar{\bH}_{\lceil\ell\rfloor}^\dagger$ ($\ell\in[q]$) and $\bar{\bar{\bH}}^\dagger$ , 
		$$\underset{1\leq i,j\leq n\atop \balpha_i\neq \balpha_j}{\max}\;\frac{\rho(\bM_{\cdot i},\, \bM_{\cdot j})}{\|\balpha_i-\balpha_j\|^{\uvarsig}}
		\lesssim_\P 1\quad \text{and}\quad 
		\underset{1\leq i,j\leq n\atop \balpha_i\neq \balpha_j}{\min}\;\frac{\rho(\bM_{\cdot i},\, \bM_{\cdot j})}{\|\balpha_i-\balpha_j\|^{\lvarsig}}\gtrsim_\P 1.$$
\end{assumption}

Next, we impose conditions for local principal component analysis that is analogous to Assumption \ref{Assumption: LPCA} in the main paper. To ease the exposition, we introduce the notation $\bH_{\subi}$, $\bar\bH_{\subi,\lceil\ell\rfloor}$ and $\bar{\bar{\bH}}_{\subi}$ that are submatrices of $\bH^\wr$,
$\bar\bH_{\lceil\ell\rfloor}^{\ddagger}$ and $\bar{\bar{\bH}}^\ddagger$ respectively, which only contain the columns of nearest neighbors of the unit $i$ obtained in the estimation procedure. In addition, $\E[\cdot|\mathcal{N}_i]$ below denotes the expectation taking the information used for matching as fixed. Note that for each of $\bH_{\subi}$, $\bar\bH_{\subi,\lceil\ell\rfloor}$ and $\bar{\bar{\bH}}_{\subi}$, $\E[\cdot|\mathcal{N}_i]$ below may have different conditioning sets.
Also, define  $\delta_{n}=(K^{1/2}\wedge p^{1/2})/\sqrt{\log (n\vee p)}$, $h_{n,\varrho}=(K/n)^{\frac{\uvarsig}{\lvarsig\bar{r}}}$, 
$h_{n,\alpha}=(K/n)^{\frac{\uvarsig}{\lvarsig r}}$.

\begin{assumption}[Local Approximation]
	\label{SA-Assumption: local approximation}\leavevmode
			For each $\bM=\bH_{\subi}, 
			\bar\bH_{\subi,\lceil\ell\rfloor} (\ell=1, \cdots, q)$ and $\bar{\bar{\bH}}_{\subi}$, 
			$\bM$ admits an $L^2$-type decomposition 
			$\bM_{\subi}=\bF_{\subi}^{\textsf{M}}(\bLambda_{\subi}^{\textsf{M}})'+\bXi_{\subi}^{\textsf{M}}+\bU_{\subi}^{\textsf{M}}$ 
			with $\bLambda_{\subi}^{\textsf{M}}\in\mathbb{R}^{K\times d_i^{\textsf{M}}}$, $\bF_{ \subi}^{\textsf{M}}=
			\E[\bM_{\subi}
			\bLambda_{\subi}^{\textsf{M}}|\mathcal{N}_i]
			\E[(\bLambda_{\subi}^{\textsf{M}})'\bLambda_{\subi}^{\textsf{M}}|\mathcal{N}_i]^{-1}$ and the following conditions satisfied:
	\begin{enumerate}[label=(\alph*)]
		\item 
		For $i=1, \cdots, n$, there exists some diagonal matrix $\bUpsilon_{\subi}^{\textsf{M}}=\diag(\upsilon_{1,\subi}^{\textsf{M}}, \cdots, \upsilon^{\textsf{M}}_{\ttd_i^{\textsf{M}},\subi})$ with 
		$\upsilon_{1,\subi}^{\textsf{M}}\geq\cdots\geq\upsilon^{\textsf{M}}_{\ttd_i^{\textsf{M}},\subi}$ such that 
		\begin{align*}
			&\underset{1\leq i\leq n}{\max}
			\|\bLambda_{\subi}^{\textsf{M}}(\bUpsilon_{\subi}^{\textsf{M}})^{-1}\|_{\max}\lesssim_\P 1,\\ 
			&\min_{1\leq i\leq n}s_{\min}\Big(\frac{1}{K}(\bUpsilon_{\subi}^{\textsf{M}})^{-1}(\bLambda_{\subi}^{\textsf{M}})'
			\bLambda_{\subi}^{\textsf{M}}(\bUpsilon_{\subi}^{\textsf{M}})^{-1}\Big)\gtrsim_\P 1\\
			&\max_{1\leq i\leq n}s_{\max}\Big(\frac{1}{K}(\bUpsilon_{\subi}^{\textsf{M}})^{-1}(\bLambda_{\subi}^{\textsf{M}})'
			\bLambda_{\subi}^{\textsf{M}}(\bUpsilon_{\subi}^{\textsf{M}})^{-1}\Big)\lesssim_\P 1.
		\end{align*}
		Either $\upsilon_{j,\subi}^{\textsf{M}}/\upsilon_{j+1,\subi}^{\textsf{M}}\lesssim 1$ or $\upsilon_{j,\subi}^{\textsf{M}}/\upsilon_{j+1,\subi}^{\textsf{M}}\rightarrow\infty$ holds for $j=1, \cdots, \ttd_i^{\textsf{M}}-1$;
		\item For some $m\leq\bar{m}$,  
		$\underset{1\leq i\leq n}{\max}\|\bXi_{\subi}^{\textsf{M}}\|_{\max}\lesssim_\P h_{n,\varrho}^m=o(\upsilon_{\ttd_i^{\textsf{M}},\subi})$ and $\delta_n^{-1}/\upsilon_{\ttd_i^{\textsf{M}},\subi}=o(1)$;
		
		\item $1\lesssim_\P\underset{1\leq i\leq n}{\min} 
		s_{\min}\Big(\frac{1}{p}(\bF_{\subi}^{\textsf{M}})'\bF_{\subi}^{\textsf{M}}\Big)\leq
		\underset{1\leq i\leq n}{\max}s_{\max}\Big(\frac{1}{p}
		(\bF_{\subi}^{\textsf{M}})'\bF_{\subi}^{\textsf{M}}\Big)\lesssim_\P 1$.
	\end{enumerate}
\end{assumption}

%%%%%%%%%%%%%%%%%%%%%%%%%%%%%%%%%%%%%%%%%%%%%%%%%%%%%%%%%%%%%%%

\subsection{Main Results}
To begin with, the following lemma derives the rate of convergence for $\widehat{\bvth}$, which makes it possible to separate the factor component of interest from others in Equation \eqref{SA-eq: general model}.

\begin{lem} \label{SA-lem: slope of covariates}
	Under Assumptions \ref{SA-Assumption: high-rank covariates}--\ref{SA-Assumption: local approximation},
	 if $(np)^{\frac{2}{\nu}}\delta_n^{-2}\lesssim 1$, then 
	$\|\widehat{\bvth}-\bvth\|\lesssim_\P \delta_n^{-1}+h_{n,\varrho}^{2m}$.
\end{lem}

\begin{remark}
	This is a by-product of our main analysis. In fact, it shows that the low-dimensional parameter in partially linear regression with a nonlinear factor structure can be consistently estimated. The rate of convergence above may not be sharp, since the calculation is simply based on the convergence rates of the underlying nonparametric estimators. 
\end{remark}

The next theorem, which is analogous to Theorems \ref{thm: IMD} and \ref{thm: uniform convergence of factors} in the main paper,  shows that the indirect matching discrepancy shrinks, and the local factors and factor loadings can be consistently estimated up to a rotation.

\begin{thm}[Local PCA with Covariates] \label{SA-thm: relevant FE}
	Under Assumptions \ref{SA-Assumption: high-rank covariates}--\ref{SA-Assumption: local approximation},
	if  $\delta_nh_{n,\varrho}^{2m}\lesssim 1$, and $(np)^{\frac{2}{\nu}}\delta_{n}^{-2}\lesssim 1$, then 
	\[
	\max_{1\leq i\leq n}
   \max_{1\leq k\leq K}
   \|\balpha_i-\balpha_{j_k(i)}\|\lesssim_\P
   (K/n)^{\uvarsig/(\lvarsig r)}
   +a_n^{1/\lvarsig},
   \]
   and
	there exists a matrix $\bR_{\subi}$ such that
	\begin{align*}
		&\max_{1\leq i\leq n}
		\|\widehat{\bF}_{\cdot k, \subi}-\bF_{\subi}(\bR_{\subi}^{-1})_{\cdot k}\|_{\max}\lesssim_\P
		(\delta_{n}^{-1}+h_{n,\alpha}^{m}+h_{n,\varrho}^{2m})\Big(\upsilon^{\bH_{\subi}}_{k,\subi}\Big)^{-1},\quad \text{for each } k\in[\ttd_i^{\bH_{\subi}}]\\
	&\max_{1\leq i\leq n}
	\|\widehat{\bLambda}_{\subi}-\bLambda_{\subi}\bR_{\subi}\|_{\max}\lesssim_\P
	\delta_{n}^{-1}+h_{n,\alpha}^{m}+h_{n,\varrho}^{2m}.
	\end{align*}
	Moreover, $1\lesssim_\P \min_{1\leq i\leq n}s_{\min}(\bR_{\subi})\leq \max_{1\leq i\leq n}s_{\max}(\bR_{\subi})\lesssim_\P 1$.
\end{thm}

%%%%%%%%%%%%%%%%%%%%%%%%%%%%%%%%%%%%%%%%%%%%%%%%%%%%%%%%%%%%%%%%%%%%%%%%%%%%%%%%%%%%%%%%%%%%%%%%%%%

\section{Further Discussion of Assumptions}
\label{SA-sec: discussion of conditions}

\subsection*{Informativeness}
As discussed in the main paper, Assumption \ref{Assumption: Matching}(b) is key for validity of $K$ nearest neighbors matching. 
Appendix \ref{sec: appendix matching} shows how it can be verified based on ``informativeness'' conditions that are specific to each distance function. We give some further discussion in this section.

We will first focus on condition (iii) in Theorem \ref{thm: IMD hom}, the key informativeness condition for Euclidean distance.
We remind readers that this condition is stated in a probabilistic sense and the randomness comes from both dimensions. 
However, if the maxima over the evaluation points are replaced by suprema over the whole support, then it no longer relies on the ``cross-sectional'' (indexed by $i$) randomness and concerns the properties of the latent functions only. 
Note that the randomness of the latent functions $(\eta_l:1\leq l\leq p)$ can be understood in several ways. For example, they could be a sample of functional random variables (f.r.v.) satisfying certain smoothness conditions. See \cite{Ferraty-Vieu_2006_book} for general discussion of functional data analysis. Alternatively, it may be generated based on a more restrictive but practically relevant specification:
$\eta_l(\balpha_i):=\eta(\bm{\varpi}_l;\balpha_i)$,
where $\eta(\cdot;\cdot)$ is a fixed function and the randomness across the $l$ dimension is induced by a sequence of random variables $(\bm{\varpi}_l:1\leq l\leq p)$ with some distribution $F_{\varpi}(\cdot)$ on $\mathcal{Z}$.
To simplify the discussion, attention will be mostly restricted to this specific case in the following discussion.

Recall that condition (iii) in Theorem \ref{thm: IMD hom} says that 
\begin{equation}\label{eq: def of nonsingularity}
	\lim_{\Delta\rightarrow 0}\limsup_{n,p^\dagger\rightarrow\infty}\;
	\P\Big\{\max_{1\leq i\leq n}\;
	\max_{j:\rho(\bH_{\cdot i}^\dagger,\bH_{\cdot j}^\dagger)<\Delta}\;
	\|\balpha_i-\balpha_j\|>\varepsilon\Big\}=0.
\end{equation}

\eqref{eq: def of nonsingularity} can be viewed as the continuity of the inverse map of $\bH_{\cdot i}^\dagger$. 
To see this, suppose that $\eta_l(\balpha_i)=\eta(\bm{\varpi}_l;\balpha_i)$, which is a function of $\bm\varpi_l$ indexed by $\balpha_i\in\mathcal{A}$. Under mild regularity conditions, the following uniform convergence can be shown:
\[
\sup_{\balpha,\balpha'\in\mathcal{A}}\Big|
\frac{1}{p^\dagger}\sum_{l\in\mathcal{R}^\dagger}\Big(\eta(\bm{\varpi}_l;\balpha)-\eta(\bm{\varpi}_l;\balpha')\Big)^2-
\E\Big[\Big(\eta(\bm{\varpi}_l;\balpha)-\eta(\bm{\varpi}_l;\balpha')\Big)^2\Big]\Big|=o_\P(1),
\]
where the expectation is taken against the distribution of $\bm{\varpi}_l$.
Then, we can safely remove the randomness arising from $\bm{\varpi}_l$ and impose conditions on the ``limit'' only. Specifically, condition \eqref{eq: def of nonsingularity} reduces to the following: for any $\varepsilon>0$, there exists $\Delta$ such that for all $\balpha,\balpha'\in\mathcal{A}$, 
\[
\int \Big(\eta(\bm{\varpi}_l;\balpha)-
\eta(\bm{\varpi}_l;\balpha')\Big)^2dF_{\varpi}(\bm{\varpi})< \Delta
\Rightarrow\|\balpha-\balpha'\|< \varepsilon,
\]
where $F_\varpi$ denotes the distribution of $\bm{\varpi}_l$ and  ``$\Rightarrow$'' means ``implies''.
Conceptually, if we define $g: \balpha\mapsto\eta(\cdot;\balpha)$ which is a map from $\mathcal{A}$ to $L_2(\mathcal{Z})$ (a set of square-integrable functions on the support $\mathcal{Z}$ of $\bm{\varpi}_l$ equipped with $L^2$-norm), then the above condition essentially says that the inverse map $g^{-1}$ exists and uniformly continuous.

\begin{exmp}[Polynomial]
	Let $\eta(\varpi_l;\alpha)=1+\varpi\alpha+\varpi^2\alpha^2$,  $\mathcal{Z}=\mathcal{A}=[0,1]$, and $F_\varpi$ be the uniform distribution. Then, for $\alpha,\alpha'\in\mathcal{A}$,
	$\int_{[0,1]}(\eta(\varpi;\alpha)-
	\eta(\varpi;\alpha'))^2dF_{\varpi}(\varpi)=
	(\alpha-\alpha',\alpha^2-(\alpha')^2)
	(\int_{[0,1]}(\varpi,\varpi^2)'(\varpi,\varpi^2)d\varpi)
	(\alpha-\alpha',\alpha^2-(\alpha')^2)'$.
	The matrix in the middle is simply one block in the Hilbert matrix with the minimum eigenvalue bounded away from zero. Then, the desired result immediately follows.
	\hfill\qedsymbol
\end{exmp}

\begin{exmp}[Trigonometric function]
	Let $\eta(\varpi;\alpha)=\sin(\pi(\varpi+\alpha))$, $\mathcal{Z}=\mathcal{A}=[0,1]$, and $F_\varpi$ be the uniform distribution. Take any two points $\alpha,\alpha'\in\mathcal{A}$ such that $\alpha\neq\alpha'$. Without loss of generality, assume $\alpha>\alpha'=0$ and $\varepsilon=\alpha-\alpha'$. Consider the following cases: when $0<\varepsilon<1/2$,  $|\eta(\varpi;\alpha)-\eta(\varpi;\alpha')|\geq
	1-\cos\pi\varepsilon$ for all $\varpi\in[0.5,1]$; and when $1/2\leq \varepsilon\leq 1$, $|\eta(\varpi;\alpha)-\eta(\varpi;\alpha')|\geq 
	\sin \pi\varpi$ for all $\varpi\in[0.5,1]$. This suffices to show that for each $\varepsilon>0$, there exists $\Delta_\epsilon>0$ such that for all $|\alpha-\alpha'|>\varepsilon$,  $\int_{[0,1]}(\eta(\varpi;\alpha)-\eta(\varpi;\alpha'))^2d\varpi>\Delta_\varepsilon$, which is simply the contrapositive of the desired result.
	\hfill\qedsymbol
\end{exmp}

\begin{remark}[Regime shift]
The ``smoothness'' of $\eta_l$ over the $l$ dimension is unnecessary in our general framework. For example, consider a simple artificial specification:
$\eta_l(\alpha)=\alpha^2+1$ for some $l=l_0\in\mathcal{R}^{\dagger}$ and $\eta_l(\alpha)=2\alpha^2+1$ for $l\neq l_0$.
Clearly, the case of $l=l_0$ is distinct from others. However, for any $\alpha,\tilde{\alpha}\in\mathcal{A}=[0,1]$ such that $|\alpha-\tilde{\alpha}|>\varepsilon$,
$\frac{1}{p^\dagger}\sum_{l\in\mathcal{R}^\dagger}
(\eta_{l}(\alpha)-\eta_{l}(\tilde{\alpha}))^2
= \frac{4(p^\dagger-1)+1}{p^\dagger}(\alpha^2-\tilde{\alpha}'^2)^2 \geq \varepsilon^4$.
Multiple regime shifts and more complex factor structures are allowed as long as there are sufficiently many ``dimensions'' in which the difference in values of $\alpha$ can be detected.
\end{remark}

Next, note that the condition described above for the squared Euclidean distance is also sufficient for the informativeness requirement corresponding to the pseudo-max distance (condition (i) in Theorem \ref{thm: IMD hsk}). To see this, suppose that 
$\sup_{\balpha,\balpha',\balpha''\in\mathcal{A}}
|\frac{1}{p^\dagger}\sum_{l\in\mathcal{R}^\dagger}(\eta(\bm{\varpi}_l;\balpha)-
\eta(\bm{\varpi}_l;\balpha'))\eta(\bm{\varpi}_l;\balpha'')-\E[(\eta(\bm{\varpi}_l;\balpha)-\eta(\bm{\varpi}_l;\balpha'))\eta(\bm{\varpi}_l;\balpha'')]|=o_\P(1)$, and note that
$$\sup_{\balpha''\in\mathcal{A}\atop \balpha''\neq \balpha,\balpha'}|\E[(\eta(\bm{\varpi}_l;
\balpha)-\eta(\bm{\varpi}_l;\balpha'))\eta(\bm{\varpi}_l;\balpha'')]|=o(1) \Rightarrow
\E[(\eta(\bm{\varpi}_l;\balpha)-\eta(\bm{\varpi}_l;\balpha'))^2]=o(1).$$ 
Combining this fact with the previous condition for the squared Euclidean distance, we can establish the informativeness requirement \eqref{eq: def of nonsingularity} with respect to the pseudo-max distance.

\subsection*{Non-collapsing}

We also imposed a technical condition, ``non-collapsing'', for the pseudo-max distance (condition (iii) in Theorem \ref{thm: IMD hsk}), which is only used to obtain a sharp bound on the indirectly matching discrepancy. We briefly discuss how to verify it in this section. 

Recall that ``non-collapsing'' requires that 
there exists an absolute constant $\underline{c}'>0$ such that
	\begin{equation}\label{eq: def of non-collapsing}
		\lim_{n,p^\dagger\rightarrow\infty}\;
		\P\Big\{
		\min_{1\leq \ell\leq r}
		\min_{1\leq i\leq n}
		\sup_{\balpha\in\mathcal{A}}
		\frac{1}{p^\dagger}\Big\|\mathscr{P}_{\balpha_i,\ell}[\bmeta(\balpha)]\Big\|^2\geq \underline{c}'\Big\}=1.
	\end{equation}
When gradient vector $\nabla\bmeta$ is not collinear, i.e., $\min_{1\leq i\leq n}s_{\min}(\nabla\bmeta(\balpha_i)
\nabla\bmeta(\balpha_i)')$ is bounded away from zero, the tangent space is well defined at every point. 
Then, letting all sample averages converge to limits,  condition \eqref{eq: def of non-collapsing} can be restated as
\[
\inf_{\balpha\in\mathcal{A}}\sup_{\tilde{\balpha}\in\mathcal{A}}\Big\|
\int\Big(\frac{\partial}{\partial \balpha}\eta(\bm{\varpi};\balpha)\Big)\eta(\bm{\varpi};\tilde{\balpha})dF_\varpi(\bm{\varpi})\Big\|\geq \underline{c}'>0.
\]
Now we consider the previous two examples.

\begin{exmp}[Polynomial, continued]
	In this scenario,
	\[
	\sup_{\tilde{\alpha}}\Big|\int_{[0,1]}\Big(\frac{d}{d\alpha}\eta(\varpi;\alpha)\Big)\eta(\varpi;\tilde{\alpha})d\varpi\Big|=
	\sup_{\tilde{\alpha}}\Big|\frac{1}{2}+\frac{\tilde{\alpha}}{3}+\frac{\tilde{\alpha}^2}{4}+\Big(\frac{2}{3}+\frac{\tilde{\alpha}}{2}+\frac{2\tilde{\alpha}^2}{5}\Big)\alpha\Big|\geq \frac{13}{12},
	\]
	where the last inequality holds by taking $\tilde{\alpha}=1$. Then, the result follows.
	\hfill\qedsymbol
\end{exmp}

\begin{exmp}[Trigonometric function, continued]
	In this scenario,
	\[
	\begin{split}
		\sup_{\tilde{\alpha}}\Big|\int_{[0,1]}\Big(\frac{d}{d\alpha}\eta(\varpi;\alpha)\Big)\eta(\varpi;\tilde{\alpha})d\varpi\Big|&=
		\sup_{\tilde{\alpha}}\Big|\int_{[0,1]}\pi\cos(\pi(\varpi+\alpha))\sin(\pi(\varpi+\tilde\alpha))d\varpi\Big|\\
		&=\pi\sup_{\tilde{\alpha}}\Big|\frac{\sin(\pi(\alpha-\tilde{\alpha}))}{2}\Big|
		\geq \pi/2,
	\end{split}
	\]
	by simply taking $|\tilde{\alpha}-\alpha|=0.5$.
	Then, the result follows.
	\hfill\qedsymbol
\end{exmp}

\subsection*{Non-degeneracy}

Theorem \ref{thm: verify LPCA} in the main paper verifies the high-level conditions in Assumption \ref{Assumption: LPCA}. The key requirement therein is the non-degeneracy of derivative vectors.
As discussed before, under mild conditions, we can make the sample average across $l$ converge and restate the condition in terms of the limit. For instance, suppose that $\mathscr{D}\bmeta_l$ contains the $0$th- and $1$st-order derivatives. Then the requirement becomes
\[
\int \Big(\mu_A(\bm{\varpi};\balpha),\,\frac{\partial}{\partial\balpha}\eta(\bm{\varpi};\balpha)\Big)\Big(\eta(\bm{\varpi};\balpha),\,\frac{\partial}{\partial\balpha}\eta(\bm{\varpi};\balpha)\Big)'dF_\varpi(\bm{\varpi})\geq c>0
\] 
uniformly over $\balpha$. We can verify this sufficient condition for the two examples discussed before.

\begin{exmp}[Polynomial, continued]
	The first-order derivative is $\frac{d}{d\alpha}\eta(\varpi;\alpha)=\varpi+2\varpi^2\alpha$. Let $\bg(\varpi;\alpha)=(1+\varpi\alpha+\varpi^2\alpha^2,\, \varpi+2\varpi^2\alpha)'$. Then,
	\begin{align*}
		\int_{[0,1]}\bg(\varpi;\alpha)\bg(\varpi;\alpha)'d\varpi&=
		\tilde{\bg}(\alpha)\Big(\int_{[0,1]}(1,\varpi,\varpi^2)'(1,\varpi,\varpi^2)d\varpi\Big)
		\tilde{\bg}(\alpha)'\\
		&\gtrsim\tilde{\bg}(\alpha)\tilde{\bg}'(\alpha),\qquad\text{for}\quad
		\tilde{\bg}(\alpha)=\bigg(\begin{array}{ccc}
			1&\alpha&\alpha^2\\
			0&1&2\alpha
		\end{array}
		\bigg).
	\end{align*}
	$\tilde{\bg}(\alpha)\tilde{\bg}(\alpha)'$ is positive definite for any $\alpha$. The coefficients of its characteristic functions are continuous on a compact support, and thus by Theorem 3.9.1 of \cite{Tyrtyshnikov_2012_book}, their eigenvalues are also continuous on the support. Then, the desired result follows.
	\hfill\qedsymbol
\end{exmp}

\begin{exmp}[Trigonometric function, continued]
	Note that $\frac{d}{d\alpha}\eta(\varpi;\alpha)=\pi\cos(\pi(\varpi+\alpha))$. Let $\bg(\varpi;\alpha)=(\sin(\pi(\varpi+\alpha)), \pi\cos(\pi(\varpi+\alpha)))'$. Then,
	\[
	\begin{split}
		&\int_{[0,1]}\bg(\varpi;\alpha)\bg(\varpi;\alpha)'d\varpi=
		\tilde{\bc}\Big(\int_{[0,1]}\tilde{\bg}(\varpi;\alpha)\tilde{\bg}(\varpi;\alpha)'d\varpi\Big)\tilde{\bc}
		=\frac{1}{2\pi}\tilde{\bc}\bigg(\begin{array}{cc}
			\pi&0\\
			0&\pi
		\end{array}\bigg)\tilde{\bc},	
		\quad\text{where}\\
		&\tilde{\bg}(\varpi;\alpha)=(\sin(\pi(\varpi+\alpha)), \cos(\pi(\varpi+\alpha)))', \quad\tilde{\bc}=\bigg(\begin{array}{cc}
			1&0\\
			0&\pi
		\end{array}
		\bigg).
	\end{split}
	\]
	Then, the desired result follows.
	\hfill\qedsymbol
\end{exmp}

%%%%%%%%%%%%%%%%%%%%%%%%%%%%%%%%%%%%%%%%%%%%%%%%%%%%%%%%%%%%%%%%%%%%%%

%%%%%%%%%%%%%%%%%%%%%%%%%%%%%%%%%%%%%%%%%%%%%%%%%%%%%%%%%%%%%%%%%%%%%%%%%%%%%%%%%%%%%%%%
\section{Proofs}\label{SA-sec: proofs}
\subsection{Proofs for Appendix \ref{sec: appendix matching}}
\subsubsection{Proof of Theorem \ref{thm: IMD hom}}
	For any pair $(i,j)$,
	$\rho(\bX^{\dagger}_{\cdot i}, \bX^{\dagger}_{\cdot j})
	=\frac{1}{p^\dagger}\|\bX^{\dagger}_{\cdot i}-\bX^{\dagger}_{\cdot j}\|^2
	=\frac{1}{p^\dagger}\|\bH^{\dagger}_{\cdot i}-\bH^{\dagger}_{\cdot j}\|^2+
	\frac{1}{p^\dagger}\|\bU^\dagger_{\cdot i}-\bU^\dagger_{\cdot j}\|^2
	+\frac{2}{p^\dagger}(\bH^{\dagger}_{\cdot i}-\bH^{\dagger}_{\cdot j})' (\bU^\dagger_{\cdot i}-\bU^\dagger_{\cdot j})$.
	For the second term,
	\begin{align*}
		\frac{1}{p^\dagger}\|\bU^\dagger_{\cdot i}-\bU^\dagger_{\cdot j}\|^2=2\sigma^2+\frac{1}{p^\dagger}\sum_{l\in\mathcal{R}^\dagger}(u_{il}^2-\sigma^2)
		+\frac{1}{p^\dagger}\sum_{l\in\mathcal{R}^\dagger}(u_{jl}^2-\sigma^2)-\frac{2}{p^\dagger}\sum_{l\in\mathcal{R}^\dagger}u_{il}u_{jl}.
	\end{align*}
	Let $\zeta_{il}:=u_{il}^2-\sigma^2$ and write $\zeta_{il}=\zeta_{il}^-+\zeta_{il}^+$ where $\zeta_{il}^-:=\zeta_{il}\I(\zeta_{il}\leq \tau_n)-\E[\zeta_{il}\I(\zeta_{il}\leq \tau_n)|\mathscr{F}]$ and $\zeta^+_{it}:=\zeta_{il}\I(\zeta_{il}>\tau_n)-\E[\zeta_{il}\I(\zeta_{il}>\tau_n)|\mathscr{F}]$ for $\tau_n=\sqrt{p/\log n}$.
	Then, for any $\delta>0$, by Bernstein's inequality,
	\begin{align*}
		\P\Big(\Big|\frac{1}{p^\dagger}\sum_{l\in\mathcal{R}^\dagger}\zeta_{il}^-\Big|>\delta
		\Big|\mathscr{F}\Big)\leq
		2\exp\bigg(-\frac{\delta^2/2}{\frac{1}{(p^\dagger)^2}\sum_{l\in\mathcal{R}^\dagger}\E[(\zeta_{il}^-)^2|\mathscr{F}]
			+\frac{1}{3p^\dagger}\tau_n\delta}\bigg).
	\end{align*}
	On the other hand,
	\[
	\P\Big(\max_{1\leq i\leq n}
	\Big|\frac{1}{p^\dagger}\sum_{l\in\mathcal{R}^\dagger}\zeta_{il}^+\Big|>\delta\Big|\mathscr{F}\Big)
	\leq n\max_{1\leq i\leq n}\frac{\sum_{l\in\mathcal{R}^\dagger}\E[(\zeta_{il}^+)^2|\mathscr{F}]}
	{(p^\dagger)^2\delta^2}
	\lesssim \frac{n}{p^\dagger\tau_n^\nu\delta^2}.
	\]
	Then, by the imposed rate restriction, $p^\dagger \asymp p$ and setting $\delta=\sqrt{\log n/p}$, it follows that
	$\max_{1\leq i\leq n}\Big|\frac{1}{p^\dagger}\sum_{l\in\mathcal{R}^\dagger}(u_{il}^2-\sigma^2)\Big|\lesssim_\P \sqrt{\frac{\log n}{p}}$.

	Apply this argument to other terms. Specifically,
	for any $i\neq j$, since $\E[u_{il}u_{jl}|\mathscr{F}]=0$, by the rate restriction,
	$\max_{i\neq j}
	\Big|\frac{1}{p^\dagger}\sum_{l\in\mathcal{R}^\dagger}u_{il}u_{jl}\Big|\lesssim_\P\sqrt{\frac{\log n}{p}}$.
	Then, 
	$\max_{i\neq j}\Big|\frac{1}{p^\dagger}\|\bU^\dagger_{\cdot i}-\bU^\dagger_{\cdot j}\|^2-2\sigma^2\Big|\lesssim_\P\sqrt{\frac{\log n}{p}}$.
	
	Similarly, by the moment condition, the rate restriction and the fact that $\E[(\eta_{l}(\balpha_i)-\eta_{l}(\balpha_j))(u_{il}-u_{jl})]=0$ for all $l$ and $i\neq j$,
	$$\max_{i\neq j}\Big|\frac{1}{p}(\bH^{\dagger}_{\cdot i}-\bH^{\dagger}_{\cdot j})'(\bU^\dagger_{\cdot i}-\bU^\dagger_{\cdot j})\Big|\lesssim_\P\Big(\frac{\log n}{p}\Big)^{1/2}.$$
	This suffices to show $a_n=(\log n/p)^{1/2}$, $\rho_0=2\sigma^2$. 
	
	Next, it follows immediately from Assumption \ref{Assumption: Regularities} that $\frac{1}{p}\|\bH^\dagger_{\cdot i}-\bH^\dagger_{\cdot j}\|^2\lesssim \|\balpha_i-\balpha_j\|^2$ for all $(i,j)$, which implies $\uvarsig=2$. On the other hand,
	by the condition imposed, 
	for any $\epsilon>0$ and $\tau>0$, there exists some $\Delta_\epsilon>0$ and $M_\epsilon>0$ such that $\P(\max_{1\leq i\leq n}\max_{\rho(\bH^\dagger_{\cdot i},\bH^\dagger_{\cdot j})<\Delta_\epsilon}\|\balpha_i-\balpha_j\|>\epsilon)<\tau/2$ for all $n,p>M_\epsilon$. 
	Then, we consider a local linearization around $\balpha_i$.
	By the condition imposed, w.p.a. 1, 
	\begin{align*}
		\|\balpha_i-\balpha_j\|^2
		&\lesssim \frac{1}{p^\dagger}\Big\|\nabla\bmeta^\dagger(\balpha_i)'(\balpha_i-\balpha_{j})+
		\frac{1}{2}(\balpha_i-\balpha_{j})'\nabla^2\bmeta(\tilde{\balpha})'(\balpha_i-\balpha_{j})\Big\|^2\\
		&=\frac{1}{p^\dagger}\|\bH^{\dagger}_{\cdot i}-\bH^{\dagger}_{\cdot j}\|^2,
	\end{align*}
	where $\nabla^2\bmeta^\dagger(\tilde{\balpha})$ is a $p^\dagger\times r\times r$ array with the $l$th sheet given by the Hessian matrix of $\eta_{l}(\cdot)$ with respect to $\balpha$ evaluated at some appropriate point $\tilde{\balpha}_{i,l}$ between $\balpha_i$ and $\balpha_{j}$, and $\tilde{\balpha}=(\tilde{\balpha}_{i,1}', \cdots, \tilde{\balpha}_{i,p}')'$.   
	Then, it follows that $\lvarsig=2$.

\subsubsection{Proof of Theorem \ref{thm: IMD hsk}}

	For any $j\neq i$ and $k\notin\{j,i\}$,
	\[
	\frac{1}{p^\dagger}(\bX^{\dagger}_{\cdot j}-\bX^{\dagger}_{\cdot i})'\bX^{\dagger}_{\cdot k}
	= \frac{1}{p^\dagger}(\bH^{\dagger}_{\cdot j}-\bH^{\dagger}_{\cdot i})'\bH^{\dagger}_{\cdot k}+
	\frac{1}{p^\dagger}(\bH^{\dagger}_{\cdot j}-\bH^{\dagger}_{\cdot i})'\bU^\dagger_{\cdot k}+
	\frac{1}{p^\dagger}(\bU^\dagger_{\cdot j}-\bU^\dagger_{\cdot i})'\bH^{\dagger}_{\cdot k}+
	\frac{1}{p^\dagger}(\bU^\dagger_{\cdot j}-\bU^\dagger_{\cdot i})'\bU^\dagger_{\cdot k}.
	\]
	We apply the truncation argument again as in the proof of Theorem \ref{thm: IMD hom}.
	Let $\zeta_{ikl}:=u_{il}u_{kl}$ and write $\zeta_{ikl}=\zeta_{ikl}^-+\zeta_{ikl}^+$ where 
	$\zeta_{ikl}^-:=\zeta_{ikl}\I(\zeta_{ikl}\leq \tau_n)-\E[\zeta_{ikl}\I(\zeta_{ikl}\leq \tau_n)|\mathscr{F}]$ and $\zeta^+_{ikl}:=\zeta_{ikl}\I(\zeta_{ikl}>\tau_n)-\E[\zeta_{ikl}\I(\zeta_{ikl}>\tau_n)|\mathscr{F}]$ for $\tau_n=\sqrt{p/\log n}$.
	Then, for any $\delta>0$, by Bernstein's inequality,
	\begin{align*}
		\P\Big(\Big|\frac{1}{p^\dagger}\sum_{l\in\mathcal{R}^\dagger}\zeta_{ikl}^-\Big|>\delta
		\Big|\mathscr{F}\Big)\leq
		2\exp\bigg(-\frac{\delta^2/2}{\frac{1}{(p^\dagger)^2}\sum_{l\in\mathcal{R}^\dagger}
			\E[(\zeta_{ikl}^-)^2|\mathscr{F}]
			+\frac{1}{3p^\dagger}\tau_n\delta}\bigg).
	\end{align*}
	On the other hand,
	\[
	\P\Big(\max_{1\leq i, k\leq n\atop i\neq k}
	\Big|\frac{1}{p^\dagger}\sum_{l\in\mathcal{R}^\dagger}\zeta_{ikl}^+\Big|>\delta\Big|\mathscr{F}\Big)
	\leq n^2\max_{1\leq i,j\leq n}\frac{\sum_{l\in\mathcal{R}^\dagger}\E[(\zeta_{ikl}^+)^2|\mathscr{F}]}
	{(p^\dagger)^2\delta^2}
	\lesssim \frac{n^2}{p^\dagger\tau_n^\nu\delta^2}.
	\]
	Then, by the rate restriction and setting $\delta=\sqrt{\log n/p}$, 
	$\max_{i\neq j}|\frac{1}{p^\dagger}\sum_{l\in\mathcal{R}^\dagger}u_{il}u_{jl}|\lesssim_\P \sqrt{\log n/p}$.
	Note that in this case the moment condition required is weaker than in Theorem \ref{thm: IMD hom}.
	By similar argument, we conclude that the last three terms in the decomposition are $\bar{O}_\P(\sqrt{\log n/p})$ uniformly over $i,j,k$, which suffices to show $\rho_0=0$ and $a_n=\sqrt{\log n/p}$.
	
	Next, for all $k\neq i,j$, by Cauchy-Schwartz inequality,
	\[
	\begin{split}
		\Big|\frac{1}{p}(\bH^{\dagger}_{\cdot j}-\bH^{\dagger}_{\cdot i})'\bH^{\dagger}_{\cdot k}\Big|
		\leq\Big(\frac{1}{p}\sum_{l\in\mathcal{R}^\dagger}\Big(\eta_{l}(\balpha_i)-\eta_{l}(\balpha_{j})\Big)^2\Big)^{1/2}
		\Big(\frac{1}{p}\sum_{l\in\mathcal{R}^\dagger}\eta_{l}(\balpha_k)^2\Big)^{1/2}
		\lesssim \|\balpha_j-\balpha_i\|.
	\end{split}
	\]
	This implies that $\uvarsig=1$.

	On the other hand, denote by $\mathcal{M}_n$ the event on which conditions (ii) and (iii) hold. Then, $\P(\mathcal{M}_n)=1-o(1)$. 
	On $\mathcal{M}_n$,
	for each $\balpha_i$, given the direction $\balpha_i-\balpha_{j}$, pick a point $\bH^{\dagger}_{\cdot\ell}=\bmeta^\dagger(\balpha_{\ell})$ such that  $\mathscr{P}_{\balpha_i}[\bmeta^\dagger(\balpha_{\ell})]=\nabla\bmeta^\dagger(\balpha_i)(r_n(\balpha_i-\balpha_{j}))$ for some $r_n$ and 
	$\frac{1}{p^\dagger}\|\mathscr{P}_{\balpha_i}[\bmeta^\dagger(\balpha_{\ell})]\|^2\geq \underline{c}>0$. It follows that 
	$\|r_n(\balpha_i-\balpha_{j})\|\geq \underline{c}'>0$ for some constant $\underline{c}'>0$. 
	Suppose first that $\ell\neq i, j_k(i)$. Then, we conclude that on $\mathcal{M}_n$,
	\[
	\underline{c}'\|\balpha_i-\balpha_{j}\|\leq
	|r_n|\|\balpha_i-\balpha_{j}\|^2
	\lesssim\, |r_n|(\balpha_i-\balpha_{j})'\Big(\frac{1}{p^\dagger}\nabla\bmeta^\dagger(\balpha_i)'\nabla\bmeta^\dagger(\balpha_i)\Big)
	(\balpha_i-\balpha_{j}).
	\]
	These inequalities hold uniformly over $i$ and $j$. 
	Note that by the second-order expansion, for some constant $\bar{c}>0$,
	\[
	\Big|\frac{1}{p^\dagger}(\bH^{\dagger}_{\cdot i}-\bH^{\dagger}_{\cdot j})'\bH^{\dagger}_{\cdot \ell}\Big|\geq|r_n|(\balpha_i-\balpha_{j})'\Big(\frac{1}{p^\dagger}\nabla\bmeta^\dagger(\balpha_i)'\nabla\bmeta^\dagger(\balpha_i)\Big)
	(\balpha_i-\balpha_{j})-\bar{c}\|\balpha_i-\balpha_{j}\|^2.
	\]
	Moreover, for each $i$ and $j$, if $\ell=i$ or $j$, then take its nearest neighbor $\ell'$ other than $i$ and $j$. Without loss of generality, consider $\ell=i$. The last step would become
	\begin{align*}
	\rho(\bH_{\cdot i}^\dagger, \bH_{\cdot j}^\dagger)+o_\P(1)\|\balpha_j-\balpha_i\|
	&\geq\Big|\frac{1}{p^\dagger}(\bH^{\dagger}_{\cdot i}-\bH^{\dagger}_{\cdot j})'\bH^{\dagger}_{\cdot \ell'}\Big|+
	\Big|\frac{1}{p^\dagger}(\bH^{\dagger}_{\cdot i}-\bH^{\dagger}_{\cdot j})'(\bH^\dagger_{\cdot i}-\bH^{\dagger}_{\cdot \ell'})
	\Big|\\
	&\geq\Big|\frac{1}{p^\dagger}(\bH^{\dagger}_{\cdot i}-\bH^{\dagger}_{\cdot j})'\bH^{\dagger}_{\cdot i}\Big|\gtrsim\|\balpha_j-\balpha_i\|.
	\end{align*}
	Then, we conclude $\lvarsig=1$.

\subsubsection{Proof of Theorem \ref{thm: dist of average}}
	Note that
	\[
	\rho(\bX^\dagger_{\cdot i}, \bX^\dagger_{\cdot j})=
	\Big|\frac{1}{p^\dagger}\sum_{l\in\mathcal{R}^\dagger}
	\Big(\eta_l(\balpha_i)+u_{il}-\eta_l(\balpha_j)-u_{jl}\Big)\Big|.
	\]
	Applying the truncation argument given before and using the fact that $\E[u_{il}|\mathscr{F}]=0$ for all $i$ and $l$, we have
	\[
	\max_{1\leq i, j\leq n}\Big|\frac{1}{p^\dagger}\sum_{l\in\mathcal{R}^\dagger}(u_{il}-u_{jl})\Big|\lesssim_\P \Big(\frac{\log n}{p}\Big)^{1/2},
	\]
	which suffices to show $\rho_0=0$ and $a_n=\sqrt{\log n/p}$.
	
	Next, since $|\frac{1}{p^\dagger}\sum_{l\in\mathcal{R}^\dagger}(\eta_l(\balpha_j)-\eta_l(\balpha_i))|\lesssim\|\balpha_j-\balpha_i\|$, we have $\uvarsig=1$. On the other hand, the inverse of $\bar{\eta}(\cdot)$ has the first derivative bounded on $\mathcal{A}$ by the condition imposed.
	Thus, $\lvarsig=1$ as well.

\subsubsection*{Proof of Theorem \ref{thm: verify LPCA}}
\begin{proof}
	We first show part (a) of Assumption \ref{Assumption: LPCA} holds.
	By Lemma \ref{lem: direct matching}, there exists a constant $\underline{c}>0$ such that w.p.a.1, $\min_{1\leq i\leq n}\max_{1\leq k\leq K}\|\balpha_i-\balpha_{j_k(i)}\|\geq \underline{c}(K/n)^{1/r}$. Also, $\max_{1\leq i\leq n}\max_{1\leq k\leq K}\|\balpha_i-\balpha_{j_k(i)}\|\lesssim_\P (K/n)^{1/r}$ by Theorem \ref{thm: IMD} and the rate condition.
	Let $\blambda(\balpha)$ be the $\ttd_i$ monomial basis of degree no greater than $m-1$ (including the constant) centered at $\balpha_i$. Then, the condition $\|\bLambda_{\subi}\bUpsilon_{\subi}^{-1}\|_{\max}\lesssim_\P 1$ immediately follows. Since $\ttd_i$ is fixed, the upper bound on the maximum singular value also follows. Regarding the lower bound on the minimum singular value, by Lemma \ref{lem: direct matching}, Theorem \ref{thm: IMD} and the conditions imposed, $\min_{1\leq i\leq n}\widehat{R}_i\geq \underline{c}'(K/n)^{1/r}$ for some absolute constant $\underline{c}'>0$ w.p.a.1, where $\widehat{R}_i$ is the radius defined in Lemma \ref{lem: conditional independence of KNN}. Then, there exists $h=\underline{c}''(K/n)^{1/r}$ for some small enough absolute constant $\underline{c}''>0$ such that w.p.a.1,   $\rho(\bH_{\cdot i}^{\dagger},\bH_{\cdot j}^{\dagger})\leq \widehat{R}_i$ for all $\|\balpha_i-\balpha_j\|\leq h$ and $i\in[n]$. On this event,
	$s_{\min}(K^{-1}\sum_{k=1}^{K}\bUpsilon_{\subi}^{-1}\blambda(\balpha_{j_k(i)})\blambda(\balpha_{j_k(i)})'\bUpsilon^{-1})\geq s_{\min}(K^{-1}\sum_{j=1}^{n}\bUpsilon_{\subi}^{-1}\blambda(\balpha_j)\blambda(\balpha_j)'\bUpsilon_{\subi}^{-1}\I(\|\balpha_i-\balpha_j\|\leq h))$.
	Since  $s_{\min}(\frac{1}{n}\sum_{j=1}^{n}\bUpsilon_{\subi}^{-1}\blambda(\balpha_j)\blambda(\balpha_j)'\\
	\bUpsilon_{\subi}^{-1}\I(\|\balpha_i-\balpha_j\|\leq h))\gtrsim h^r$ w.p.a. 1, the desired lower bound follows.

	Next, we consider part (c). Conditional on $\widehat{R}_i$, $\{\blambda(\balpha_{j_k(i)}):1\leq k\leq K\}$ is a bounded independent sequence. Then, by Bernstein inequality, we have
	$\max_{i\in[n]}\Big|\frac{1}{K}\bUpsilon_{\subi}^{-1}\bLambda_{\subi}'\bLambda_{\subi}\bUpsilon_{\subi}^{-1}
	- \E^\ddagger[\bUpsilon_{\subi}^{-1}\blambda(\balpha_{j_k(i)})\blambda(\balpha_{j_k(i)})'\bUpsilon_{\subi}^{-1}]\Big|=o_\P(1)$.
	By Assumption \ref{Assumption: Regularities} and Taylor expansion,
	$$\max_{l\in\mathcal{R}^\ddagger}\max_{i\in [n]}\max_{j\in\mathcal{N}_i}
	\Big|\eta_{l}(\balpha_j)-\blambda(\balpha_j)'\tilde{\bbeta}_{l,\subi}\Big|\lesssim_\P h_{n}^m,$$
	where $\tilde{\bbeta}_{l,\subi}$ is a vector of derivatives in the Taylor expansion.
	Let $\tilde{r}_{l,\subi}(\balpha_j):=\eta_{l}(\balpha_j)-
	\blambda(\balpha_j)'\tilde{\bbeta}_{l,\subi}$, and let
	$\bbeta_{l,\subi}$ be the coefficients of the $L^2$-projection of $\eta_{l}(\cdot)$ onto the space spanned by $\blambda(\cdot)$ (so $\bbeta_{l,\subi}$'s are the row vectors of the factor matrix $\bF_{ \subi}$). 
	Then, 
	$\bbeta_{l,\subi}=\tilde{\bbeta}_{l,\subi}+
	\E^\ddagger[\blambda(\balpha_{j_k(i)})\blambda(\balpha_{j_k(i)})']^{-1}\E^\ddagger[\blambda(\balpha_{j_k(i)})\tilde{r}_{l,\subi}(\balpha_{j_k(i)})]
	=:\tilde{\bbeta}_{l,\subi}+\Delta_{l,\subi}$.
	Noting the fact that 
	$\bUpsilon_{\subi}^{-1}\E^\ddagger[\blambda(\balpha_{j_k(i)})\blambda(\balpha_{j_k(i)})']\bUpsilon_{\subi}^{-1}\gtrsim 1$ uniformly over $i$ w.p.a. 1,
	$\bUpsilon_{\subi}^{-1}\blambda(\balpha_{j_k(i)})\lesssim 1$ w.p.a.1, and $\min_{j}\upsilon_{j,\subi}\asymp h_{n}^{m-1}$,
	we have that $\max_{i\in[n]}\max_{l\in\mathcal{R}^\ddagger}|\Delta_{l,\subi}|=o_\P(1)$. Thus, the result in part (b) follows.
	
	Finally, for part (b), note that 
	\begin{small}
	$$\eta_{l}(\balpha_{j_k(i)})-\blambda(\balpha_{j_k(i)})'\bbeta_{l,\subi}
	=\tilde{r}_{l,\subi}(\balpha_{j_k(i)})-\blambda(\balpha_{j_k(i)})'\E^\ddagger[\blambda(\balpha_{j_k(i)})\blambda(\balpha_{j_k(i)})']^{-1}\E^\ddagger[\blambda(\balpha_{j_k(i)})\tilde{r}_{l,\subi}(\balpha_{j_k(i)})].$$
\end{small}

	\noindent Using the argument for part (c) again, we can see that the second term is bounded by $Ch_{n}^m$ uniformly over $i$ and $l$ w.p.a.1. Then, the proof is complete.	
\end{proof}

%%%%%%%%%%%%%%%%%%%%%%%%%%%%%%%%%%%%%%%%%%%%%%%%%%%%%%%%%%%%%%%%%%%%%%%%

\subsection{Proofs for Appendix \ref{sec: appendix proofs}}

\subsubsection{Proof of Lemma \ref{lem: direct matching}}
	Let $U_K(\balpha_0)=\max_{1\leq k\leq K}\|\balpha_{j_k^*(\balpha_0)}-\balpha_0\|$. Define a cube around $\balpha_0$: $\mathcal{H}_\zeta(\balpha_0)=[\balpha_0-\zeta,\, \balpha_0+\zeta)\cap\mathcal{A}$, where $\zeta=(\frac{C'K}{\underline{f}_{\alpha}n})^{1/r}$ for some absolute constant $C'>1$ and $\underline{f}_{\alpha}$ denotes the minimum of the density of $\balpha_i$. Let $F$ and $F_n$ denote the population and empirical distribution functions for $\balpha_i$ respectively. Since the density is strictly positive, 
	$\inf_{\balpha_0\in\mathcal{A}}F(\mathcal{H}_\zeta(\balpha_0))\geq \min\{\underline{f}_{\alpha} \zeta^r, 1\}>\frac{K}{n}$.
	On the other hand,
	\begin{align*}
		&\P\Big(\sup_{\balpha_0\in\mathcal{A}}U_K(\balpha_0)>\zeta\Big)\\
		\leq &\,\P\bigg(\exists \balpha_0\in\mathcal{A}, F_n\Big(\mathcal{H}_\zeta(\balpha_0)\Big)<\frac{K}{n}\bigg)\\
		\leq&\,\P\bigg(\exists \balpha_0\in\mathcal{A}, \Big|F_n\Big(\mathcal{H}_\zeta(\balpha_0)\Big)-F\Big(\mathcal{H}_\zeta(\balpha_0)\Big)\Big|>F\Big(\mathcal{H}_\zeta(\balpha_0)\Big)
		-\frac{K}{n}\bigg)\\
		\leq&\,\P\bigg(\sup_{\balpha_0\in\mathcal{A}} \Big|F_n\Big(\mathcal{H}_\zeta(\balpha_0)\Big)-F\Big(\mathcal{H}_\zeta(\balpha_0)\Big)\Big|>\min\Big\{\frac{(C'-1)K}{n},1-\frac{K}{n}\Big\}\bigg).
	\end{align*}
	Define the oscillation modulus $\omega_n(\varepsilon):=\sup_{\balpha_0\in\mathcal{A}}
	\sqrt{n}[F_n(\mathcal{H}_{\varepsilon}(\balpha_0))-F(\mathcal{H}_\varepsilon(\balpha_0))]$.
	By \citet[Theorem 2.3]{Stute_1984_AoP}, if $\frac{(n/K)\log (n/K)}{n}=o(1)$
	and $\frac{K\log n}{n}=o(1)$, then
	$\omega_n(\zeta)\lesssim_\P\sqrt{\zeta^{r}\log \zeta^{-r}}$.
	This suffices to show that the probability on the last line goes to zero.
	
	On the other hand, since the density of $\balpha_i$ is bounded from above as well, it follows similarly that $\inf_{\balpha_0\in\mathcal{A}}U_K(\balpha_0)\geq c(K/n)^{1/r}$ w.p.a. $1$. Thus, we have proved the first result.

	Next, by definition, $\max_{1\leq k\leq K}\|\balpha_i-\balpha_{j_k(i)}\|\geq \max_{1\leq k\leq K}\|\balpha_i-\balpha_{j^*_k(\balpha_i)}\|$. Then,  the second result follows immediately.

\subsubsection{Proof of Lemma \ref{lem: conditional independence of KNN}}
	Let $f_{\widehat{R}_i}(\cdot)$ be the density of $\widehat{R}_i$ and $\delta(z, \mathscr{A})$ be an indicator function that is equal to one if $z\in \mathscr{A}$. We have already defined the set of indices for the $K$ nearest neighbors of unit $i$. Now define $\{j_k(i): K+1\leq k\leq n\}$ as the set of units that are outside the neighborhood of $\bX^{\dagger}_{\cdot i}$ of radius $\widehat{R}_i$, arranged according to the original ordering of $\{\bX^{\dagger}_{\cdot i}: 1\leq i\leq n\}$. For $\widehat{R}_i=r$, define $\mathcal{S}_r=\{\bz: \rho(\bz, \bX^{\dagger}_{\cdot i})<r\}$.
	Notice that a generic unit $j$ is included in $\mathcal{N}_i$ if and only if $\rho(\bX^{\dagger}_{\cdot i}, \bX^{\dagger}_{\cdot j})\leq \widehat{R}_i$.
	Since the original sequence $\{\bX^{\dagger}_{\cdot i}:1\leq i\leq n\}$ is i.i.d. across $i$, the joint density of $\{\balpha_{j_k(i)}: 1\leq k\leq n\}$ is
	\[
	\begin{split}
		f(\bv_1, \cdots, \bv_{K-1};\bw_{K+1}, \cdots, \bw_{n};\bz)
		=n\binom{n-1}{K-1}\prod_{k=1}^{K-1}f_\alpha(\bv_k)\int f_{X|\alpha}(\ba_{k}|\bv_k)\delta(\ba_{k}, \mathcal{S}_{\widehat{R}_i})d\ba_{k}&\\
		\times\prod_{\ell=K+1}^{n}f_\alpha(\bw_\ell)
		\int f_{X|\alpha}(\ba_{\ell}|\bw_\ell)\delta(\ba_{\ell}, \bar{\mathcal{S}}_{\widehat{R}_i}^c)d\ba_{\ell}
		\times f_\alpha(\bz)\int f_{X|\alpha}(\ba|\bz)\delta(\ba, \partial \mathcal{S}_{\widehat{R}_i})d\ba&,
	\end{split}
	\]
	where $f_\alpha(\cdot)$ is the density of $\balpha_i$, $f_{X|\alpha}(\cdot|\cdot)$ denotes the density of $\bX^{\dagger}_{\cdot i}$ conditional on $\balpha_i$ and $\widehat{R}_i$. $\bar{\mathcal{S}}_{\widehat{R}_i}^c$ is the complement of the closure of $\mathcal{S}_{\widehat{R}_i}$ and $\partial \mathcal{S}_{\widehat{R}_i}$ denotes the boundary of $\mathcal{S}_{\widehat{R}_i}$. On the other hand, the density of $\widehat{R}_i$ is
	\[
	n\binom{n-1}{K-1}G(r)^{K-1}(1-G(r))^{n-K}G'(r), \quad G(r)=\P\Big(\{\bX^{\dagger}_{\cdot j}: \rho(\bX^{\dagger}_{\cdot j}, \bX^{\dagger}_{\cdot i})<r\}\Big).
	\]
	According to the above results, $\{\balpha_{j_k(i)}:1\leq k\leq n\}$ is independent across $k$ conditional on $\widehat{R}_i$ and $\bX^{\dagger}_{\cdot i}$ with the joint conditional density given by
	\[
	\begin{split}
		G'(r)^{-1}f_\alpha(\bz)\int f_{X|\alpha}(\ba|\bz)\delta(\ba, \partial \mathcal{S}_{\widehat{R}_i})d\ba\times
		\prod_{k=1}^{K-1}G(r)^{-1}f_\alpha(\bv_k)
		&\int f_{X|\alpha}(\ba_{k}|\bv_k)\delta(\ba_{k}, \mathcal{S}_{\widehat{R}_i})d\ba_{k}\\
		\times\prod_{\ell=K+1}^{N}(1-G(r))^{-1}f_\alpha(\bw_\ell)
		&\int f_{X|\alpha}(\ba_{\ell}|\bw_\ell)\delta(\ba_{\ell}, \bar{\mathcal{S}}_{\widehat{R}_i}^c)d\ba_{\ell}.
	\end{split}
	\]

\subsubsection{Proof of Lemma \ref{lem: operator norm of eps}}

	Note $\bU_{\subi}$ is a $p^\ddagger\times K$ random matrix. Let $\mathscr{M}=\{\widehat{R}_i\}_{i=1}^n\cup\mathscr{F}$. 
	By Assumption \ref{Assumption: Matching} and the row-wise sample splitting, conditional on $\widehat{R}_i$, 
	$\bU_{\subi}$ has independent columns with mean zero, $\E[\bU_{\cdot k, \subi}(\bU_{\cdot k, \subi})'|\mathscr{M}]=\bSigma_{k,\subi}$ for all $1\leq k\leq K$ and $1\leq i\leq n$, and  $\underset{1\leq i\leq n}{\max}\|\bSigma_{\subi}\|\lesssim_\P 1$ for $\bSigma_{\subi}:=\frac{1}{K}\sum_{k=1}^{K}\bSigma_{k,\subi}$. 
	Write 
	$\frac{1}{K}\sum_{k=1}^{K}\Big(\bU_{\cdot k,\subi}
	\bU_{\cdot k, \subi}'-\bSigma_{k,\subi}\Big)=
	\frac{1}{K}\sum_{k=1}^{K}(\bH_k+\bT_k)$,
	where 
	\begin{align*}
		&\bG_k:=\bU_{\cdot k,\subi}\bU_{\cdot k,\subi}'\I(\|\bU_{\cdot k,\subi}\|^2\leq Cp)-\E[\bU_{\cdot k,\subi}\bU_{\cdot k,\subi}'\I(\|\bU_{\cdot k,\subi}\|^2\leq Cp)|\mathscr{M}],\\
		&\bT_k:=\bU_{\cdot k,\subi}\bU_{\cdot k,\subi}'\I(\|\bU_{\cdot k,\subi}\|^2> Cp)-\E[\bU_{\cdot k,\subi}\bU_{\cdot k,\subi}'\I(\|\bU_{\cdot k,\subi}\|^2> Cp)|\mathscr{M}]
	\end{align*}
	for some $C>0$. 
	For the truncated part $\bG_k$, by Bernstein's inequality for matrices and union bounds,
	for all $\tau>0$,
	\[
	\P\Big(\max_{1\leq i\leq n}\Big\|\frac{1}{K}\sum_{k=1}^{K}\bG_k\Big\|>\tau\Big|\mathscr{M}\Big)\leq
	np\exp\Big(-\frac{\tau^2/2}{Cp/K+Cp\tau/3K}\Big),
	\]
	which suffices to show that $\underset{1\leq i\leq n}{\max}\|\frac{1}{K}\sum_{k=1}^{K}\bG_k\|\lesssim_\P\max\{\sqrt{\log(n\vee p)}(p/K)^{1/2},\log(n\vee p)p/K\}$.
	On the other hand, for the tails,
	\[
	\P\Big(\max_{1\leq i\leq n}\Big\|\frac{1}{K}\sum_{k=1}^{K}\bT_k\Big\|>\tau\Big|\mathscr{M}\Big)\leq
	\P\Big(\max_{1\leq i\leq n}\|\bU^\ddagger_{ \cdot i}\|^2>Cp|\mathscr{M}\Big).
	\]
	It will be shown later that the right-hand side can be made arbitrarily small by choosing a sufficiently large but fixed $C>0$ (not varying as $n$ increases).
	Then, we conclude that $\underset{1\leq i\leq n}{\max}\|\frac{1}{K}\bU_{\subi}\bU_{\subi}'-\bSigma_{\subi}\|\lesssim_\P
	\max\{\sqrt{\log(n\vee p)}(p/K)^{1/2},\log(n\vee p)p/K\}$.
	Combining this with the bound on $\bSigma_{\subi}$, we get
	$\underset{1\leq i\leq n}{\max}\|\bU_{\subi}\|\lesssim_\P \sqrt{K}+\sqrt{p\log(n\vee p)}$.
	
	In the end, we show the uniform convergence of the second moment of $\bU_{\cdot k,\subi}$ to complete the proof.  
	Let $\zeta_{il}:=u_{il}^2-\sigma_{il}^2$, $\sigma_{il}^2=\E[u_{il}^2|\mathscr{M}]$ and write $\zeta_{il}=\zeta_{il}^-+\zeta_{il}^+$ where $\zeta_{il}^-:=\zeta_{il}\I(\zeta_{il}\leq \tau_n^2)-\E[\zeta_{il}\I(\zeta_{il}\leq \tau_n^2)]$ and $\zeta^+_{il}:=\zeta_{il}\I(\zeta_{il}>\tau_n^2)-\E[\zeta_{il}\I(\zeta_{il}>\tau_n^2)]$ for $\tau_n\asymp(n\sqrt{p}/\sqrt{\log n})^{1/(1+\nu)}$.
	Then, for any $\delta>0$, by Bernstein's inequality,
	\begin{align*}
		\P\Big(
		\Big|\frac{1}{p^\ddagger}\sum_{l\in\mathcal{R}^\ddagger}\zeta_{il}^-\Big|>\delta|\mathscr{M}\Big)\leq
		2\exp\bigg(-\frac{\delta^2/2}{\frac{\tau_n^2}{(p^\ddagger)^2}\sum_{l\in\mathcal{R}^\ddagger}\E[|\zeta_{il}^-||\mathscr{M}]
			+\frac{1}{3p^\ddagger}\tau_n^2\delta}\bigg).
	\end{align*}
	On the other hand, by Markov's inequality,
	\[
	\P\Big(\max_{1\leq i\leq n}
	\Big|\frac{1}{p^\ddagger}\sum_{l\in\mathcal{R}^\ddagger}\zeta_{il}^+\Big|>\delta|\mathscr{M}\Big)
	\leq n\max_{1\leq i\leq n}\frac{\sum_{l\in\mathcal{R}^\ddagger}\E[|\zeta_{il}^+||\mathscr{M}]}
	{p^\ddagger\delta}
	\lesssim \frac{n}{\tau_n^\nu\delta}.
	\]
	Set $\delta^2=Cn^{2/(\nu+1)}(\log n)^{\nu/(\nu+1)} /p^{\nu/(\nu+1)}$ for $C>0$ large enough. 
	Then, $\underset{1\leq i\leq n}{\max}
	|\frac{1}{p^\ddagger}\underset{l\in\mathcal{R}^\ddagger}{\sum}\zeta_{il}|\\\lesssim_\P\delta\rightarrow 0$ by the rate condition. Since  $\underset{1\leq i\leq n}{\max}\,
	\frac{1}{p}\underset{l\in\mathcal{R}^\ddagger}{\sum}\sigma_{il}^2\lesssim 1$ a.s., the desired result follows.

\subsubsection{Proof of Lemma \ref{lem: consistency eigenstructure}}

Recall that in the paper we partition $\ttd_i$ leading approximation terms into $g_i$ groups, which is identical to a partition of index set: 
$[ \ttd_i]=\cup_{\ell=0}^{g_i-1}\mathcal{C}_{i\ell}$ with $|\mathcal{C}_{i\ell}|=\ttd_{i\ell}$, where for any $j,k\in\mathcal{C}_{i\ell}$, $\upsilon_{j,\subi}\asymp\upsilon_{k,\subi}$, and for any $j\in\mathcal{C}_{i\ell}$ and $k\in\mathcal{C}_{i(\ell+1)}$, $\upsilon_{k,\subi}/\upsilon_{j,\subi}=o(1)$. 
The eigenvalues and eigenvectors are grouped accordingly. 
Now, we first prove the following lemma regarding the ``zero-order'' eigenvalues and eigenvectors.

\begin{lem} \label{lem: eigenstructure 1st order}
	Under Assumptions \ref{Assumption: Regularities}, \ref{Assumption: Matching} and \ref{Assumption: LPCA}, if $\frac{n^{\frac{2}{\nu}}\log n}{p}\lesssim 1$ and 
	$\frac{(np)^{\frac{2}{\nu}}(\log (n\vee p))^{\frac{\nu-2}{\nu}}}{K}\lesssim 1$, 
	then 
	\begin{enumerate}[label=(\roman*)]
		\item $\underset{1\leq i\leq n}{\max}\;|\widehat{\omega}_{j,\subi}/\omega_{j,\subi}-1|=o_\P(1)$, for $j\in\mathcal{C}_{i0}$; 
		\item There exists a matrix $\tilde{\bR}_{\subi}$ such that
		$\max_{1\leq i\leq n}
		\frac{1}{\sqrt{p}}\|\widehat{\bF}_{\gr{0},\subi}-\bF_{\subi}\tilde{\bR}_{\gr{0},\subi}\|_{\mathtt{F}}\lesssim_\P \delta_{n}^{-1}+h_{n}^{2m}$; 
		\item $\underset{1\leq i\leq n}{\max}\;
		\|\bM_{\widehat{\bF}_{\gr{0},\subi}}-\bM_{\bF_{\gr{0},\subi}}\|_{\mathtt{F}}\lesssim_\P\delta_{n}^{-1}+
		(\upsilon_{\bar\ttd_{i1}, \subi})^2$.
	\end{enumerate}
\end{lem}
\begin{proof}
	(i):
	Noting the following decomposition
	\[
	\begin{split}
		\bX_{\subi}\bX_{\subi}'
		=\,&\bF_{\subi}\bLambda_{\subi}'\bLambda_{\subi}\bF_{\subi}'+
		(\bXi_{\subi}+\bU_{\subi})(\bXi_{\subi}+\bU_{\subi})'+\\
		&\bF_{\subi}\bLambda_{\subi}'(\bXi_{\subi}+\bU_{\subi})'+
		(\bXi_{\subi}+\bU_{\subi})\bLambda_{\subi}\bF_{\subi}'
		=:\bG_1+\bG_2+\bG_3+\bG_4,
	\end{split}
	\]
	by Weyl's theorem, for $j=1, \cdots, \ttd_{i0}$, 
	\[
	s_j(\bG_1)+s_{\min}(\bG_2+\bG_3+\bG_4)\leq s_j(\bG_1+\cdots+\bG_4)\leq
	s_j(\bG_1)+s_{\max}(\bG_2+\bG_3+\bG_4).
	\]
	
	First, 
	$s_j(\bG_1)=s_j(
	\bLambda_{\subi}\bF_{\subi}'\bF_{\subi}\bLambda_{\subi}')$.
	By Assumption \ref{Assumption: LPCA}, 
	$s_j(\frac{1}{pK}\bG_1)\asymp_\P \upsilon_{j,\subi}$  for $j=1,\cdots, \ttd_{i0}$ and all $\subi$.
	
	Second, for $\bG_2$, we analyze the eigenvalue of each component. By Assumption \ref{Assumption: LPCA}, 
	$\underset{1\leq i\leq n}{\max}\|\frac{1}{pK}\bXi_{\subi}\bXi_{\subi}'\|\lesssim_\P h_{n}^{2m}$. 
	By Lemma \ref{lem: operator norm of eps},
	$\underset{1\leq i\leq n}{\max}\|\frac{1}{pK}\bU_{\subi}\bU_{\subi}'\|\lesssim_\P \log (n\vee p)K^{-1}+p^{-1}$. 
	By Cauchy-Schwarz inequality, $\underset{1\leq i\leq n}{\max}\|\frac{1}{pK}(\bU_{\subi}\bXi_{\subi}'+\bXi_{\subi}\bU_{\subi}')\|\lesssim_\P (\log^{1/2}(p\vee n)K^{-1/2}+p^{-1/2})h_n^m$.
	Thus, $\|\frac{1}{pK}\bG_2\|\lesssim_\P h_n^{2m}+\log(p\vee n)K^{-1}+p^{-1}$ for all $\subi$.
	
	Third, for $\bG_3+\bG_4$, note that 
	$$\Big\|\frac{1}{pK}\bF_{\subi}\bLambda_{\subi}'\bU_{\subi}'\Big\|
	\leq\frac{1}{\sqrt{K}}\frac{1}{\sqrt{p}}\|\bF_{\subi}\|
	\Big\|\frac{1}{\sqrt{p}}
	\Big(\frac{1}{\sqrt{K}}\sum_{k=1}^{K} \blambda_{j_k(i)}(\bU^\ddagger_{ \cdot j_k(i)})'\Big)\Big\|$$
	and $\underset{1\leq i\leq n}{\max}\|\bF_{\subi}\|\lesssim_\P\sqrt{p}$. Furthermore, conditional on $\widehat{R}_i$ and $\mathscr{F}$, $u_{j_k(i)l}$ is independent over $1\leq k\leq K$ and $l\in\mathcal{R}^\ddagger$, and $\underset{1\leq i\leq n}{\max}\|\bLambda_{\subi}\|_{\max}\lesssim_\P 1$. Applying Bernstein inequality combined with the truncation argument used before leads to $\underset{1\leq i\leq n}{\max}\|\frac{1}{pK}\bF_{\subi}\bLambda_{\subi}'\bU_{\subi}'\|\lesssim_\P \sqrt{\log (n\vee p)}K^{-1/2}$.
	On the other hand, $\bLambda_{\subi}$ is uncorrelated with $\bXi_{\subi}$ across $1\leq i\leq K$ by construction, and applying Bernstein inequality leads to
	$\underset{1\leq i\leq n}{\max}\frac{1}{pK}\|\bF_{\subi}\bLambda_{\subi}'\bXi_{\subi}\|\lesssim_\P \sqrt{\log (n\vee p)}h_{n}^{m}/\sqrt{K}$.
	The above fact suffices to show that
	$$\Big\|\frac{1}{pK}(\bG_3+\bG_4)\Big\|\lesssim_\P \sqrt{\log (n\vee p)}(K^{-1/2}+K^{-1/2}h_{n}^{m}).$$ 
	Then, the desired result for eigenvalues follows.
	\medskip
	
	(ii): Use the following decomposition:
	\begin{align}
		\widehat{\bF}_{\subi}-\bF_{\subi}\tilde{\bR}_{\subi}
		=\bigg\{&\frac{1}{pK}\bF_{\subi}\bLambda_{\subi}'\bU_{\subi}'\widehat{\bF}_{\subi}+
		\frac{1}{pK}\bU_{\subi}\bLambda_{\subi}\bF_{\subi}' \widehat{\bF}_{\subi}+
		\frac{1}{pK}\bF_{\subi}\bLambda_{\subi}'\bXi_{\subi}'\widehat{\bF}_{\subi}+\nonumber\\
		&\frac{1}{pK}\bXi_{\subi}\bLambda_{\subi}\bF_{\subi}'\widehat{\bF}_{\subi}+
		\frac{1}{pK}\bXi_{\subi}\bU_{\subi}'\widehat{\bF}_{\subi}+
		\frac{1}{pK}\bU_{\subi}\bXi_{\subi}'\widehat{\bF}_{\subi}+\nonumber\\
		&\frac{1}{pK}\bXi_{\subi}\bXi_{\subi}'\widehat{\bF}_{\subi}+
		\frac{1}{pK}\bU_{\subi}\bU_{\subi}'\widehat{\bF}_{\subi}
		\bigg\}\times \widehat{\bOmega}_{\subi}^{-1} \label{eq: decomposition}
	\end{align}
	where $\tilde{\bR}_{\subi}=\frac{\bLambda_{\subi}'\bLambda_{\subi}}{K}
	\frac{\bF_{\subi}'\widehat{\bF}_{\subi}}{p}\widehat{\bOmega}_{\subi}^{-1}$.
	Accordingly, a generic entry of $(\widehat{\bF}_{\subi}-\bF_{\subi}\tilde{\bR}_{\subi})$ with the row index $t\in\mathcal{R}^\ddagger$ and the column index $\ell\in[\ttd_i]$ can be written as 
	$(J_1+\cdots J_8)/\widehat{\omega}_{\ell,\subi}$ where
	{\footnotesize
		\begin{alignat*}{2}
			&J_1=\frac{1}{p}\sum_{s\in\mathcal{R}^\ddagger}\bF_{t\cdot,\subi}\Big(\frac{1}{K}\sum_{k=1}^{K}\blambda_{j_k(i)}u_{j_k(i)s}\Big)\widehat{f}_{s \ell,\subi},\qquad
			&&J_2=\Big(\frac{1}{K}\sum_{k=1}^{K}u_{j_k(i)t}\blambda_{j_k(i)}'\Big)
			\Big(\frac{1}{p}\sum_{s\in\mathcal{R}^\ddagger}\bF_{s\cdot,\subi}'\widehat{f}_{s\ell,\subi}\Big),\\
			&J_3=\frac{1}{p}\sum_{s\in\mathcal{R}^\ddagger}\bF_{t\cdot,\subi}\Big(\frac{1}{K}\sum_{k=1}^{K}\blambda_{j_k(i)}\xi_{j_k(i)s}\Big)\widehat{f}_{s\ell,\subi},
			&&J_4=\Big(\frac{1}{K}\sum_{k=1}^{K}\xi_{j_k(i)t}\blambda_{j_k(i)}'\Big)
			\Big(\frac{1}{p}\sum_{s\in\mathcal{R}^\ddagger}\bF_{s\cdot,\subi}'\widehat{f}_{s\ell,\subi}\Big),\\
			&J_5=\frac{1}{p}\sum_{s\in\mathcal{R}^\ddagger}
			\Big(\frac{1}{K}\sum_{k=1}^{K}\xi_{j_k(i)t}u_{j_k(i)s}\Big)\widehat{f}_{s\ell,\subi},
			&&J_6=\frac{1}{p}\sum_{s\in\mathcal{R}^\ddagger}
			\Big(\frac{1}{K}\sum_{k=1}^{K}u_{j_k(i)t}\xi_{j_k(i)s}\Big)\widehat{f}_{s\ell,\subi},\\
			&J_7=\frac{1}{p}\sum_{s\in\mathcal{R}^\ddagger}
			\Big(\frac{1}{K}\sum_{k=1}^{K}\xi_{j_k(i)t}\xi_{j_k(i)s}\Big)\widehat{f}_{s\ell,\subi},
			&&J_8=\frac{1}{p}\sum_{s\in\mathcal{R}^\ddagger}
			\Big(\frac{1}{K}\sum_{k=1}^{K}u_{j_k(i)t}u_{j_k(i)s}\Big)\widehat{f}_{s\ell,\subi},
		\end{alignat*}
	}
	
	\noindent and $\widehat{f}_{s\ell,\subi}$ is the $(s,\ell)$th entry of $\widehat{\bF}_{\subi}$.
	
	For $J_1$, first note that
	by assumption $\|\frac{1}{p}\sum_{t\in\mathcal{R}^\ddagger}\bF_{t\cdot,\subi}'\bF_{t\cdot,\subi}\|\lesssim_\P 1$ and $\frac{1}{p^\ddagger}\sum_{s\in\mathcal{R}^\ddagger}\widehat{f}_{s\ell, \subi}^2=1$.
	Also, 
	$\E^\ddagger[\frac{1}{K}\sum_{k=1}^{K}{\blambda}_{j_k(i)}u_{j_k(i)s}]=0$
	and
	$\E^\ddagger[\|\frac{1}{K}\sum_{k=1}^{K}\blambda_{j_k(i)}u_{j_k(i)s}\|^2]
	\lesssim_\P K^{-1}$, 
	which suffice to show that $J_1\lesssim \sqrt{\log (n\vee p)}K^{-1/2}$ by the truncation argument given in the proof of Theorem \ref{thm: IMD hsk}.
	$J_2$ can be treated similarly.	
	
	For $J_3$,
	by definition of $\bF_{\subi}$, $\E^\ddagger[\frac{1}{K}\sum_{k=1}^{K}\blambda_{j_k(i)}\xi_{j_k(i)s}]=0$, for all $s\in\mathcal{R}^\ddagger$, and $\|\bXi_{\subi}\|_{\max}\lesssim h_{n}^m$.  Thus,
	$J_3\lesssim_\P \sqrt{\log (n\vee p)}K^{-1/2}h_{n}^{m}$. $J_4$ is treated similarly.
	
	For $J_5$, $\frac{1}{p}\widehat{\bF}_{\subi}'\widehat{\bF}_{\subi}\lesssim_\P 1$, 
	$\E^\ddagger[\frac{1}{K}\sum_{k=1}^{K}\xi_{j_k(i)t}u_{j_k(i)s}]=0$,
	and
	$\E^\ddagger[(\frac{1}{K}\sum_{k=1}^K \xi_{j_k(i)t}u_{j_k(i)s})^2]\\
	\lesssim_\P K^{-1}h_{n}^{2m}$.
	Then, $J_5\lesssim_\P \sqrt{\log (n\vee p)}K^{-1/2}h_{n}^{m}$. $J_6$ can be treated similarly.
	
	For $J_7$, using the bound on $\bXi_{\subi}$, it is immediate to see $J_7\lesssim_\P h_n^{2m}$.
	For $J_{8,t}:=J_8$, it is easy to see that by Lemma \ref{lem: operator norm of eps},
	$\frac{1}{p}\sum_{t\in\mathcal{R}^\ddagger}J_{8,t}^2=
	\frac{1}{p^3K^2}\widehat{\bF}_{\cdot\ell,\subi}'\bU_{\subi}\bU_{\subi}'\bU_{\subi}\bU_{\subi}'\widehat{\bF}_{\cdot\ell,\subi}
	\lesssim_\P \delta_{n}^{-4}$.
	
	Therefore, we conclude that  
	$\frac{1}{p}\|\widehat{\bF}_{\gr{0},\subi}-\bF_{\subi}\tilde{\bR}_{\gr{0},\subi}\|_{\mathtt{F}}^2\lesssim_\P\delta_{n}^{-2}+h_{n}^{4m}$.
	\medskip
	
	(iii):
	Define a rotation matrix $\tilde{\bR}_{0,\subi}=\frac{\bLambda_{\gr{0},\subi}'\bLambda_{\gr{0},\subi}}{K}
	\frac{\bF_{\gr{0},\subi}'\widehat{\bF}_{\gr{0},\subi}}{p}\widehat{\bOmega}_{0,\subi}^{-1}$, where $\widehat{\bOmega}_{0,\subi}$ is the diagonal matrix of the leading $\ttd_{i0}$ eigenvalues of $\frac{1}{pK}\bX_{\subi}\bX_{\subi}'$. By the same argument in (ii),
	\[
	\frac{\widehat{\bF}_{\gr{0},\subi}'\bF_{\gr{0},\subi}}{p}\frac{\bLambda_{\gr{0},\subi}'\bLambda_{\gr{0},\subi}}{K}\frac{\bF_{\gr{0},\subi}'\widehat{\bF}_{\gr{0}}}{p}
	=\diag\{\widehat{\omega}_{1, \subi}, \cdots, \widehat{\omega}_{\ttd_{i0}, \subi}\}+o_\P(1).
	\]
	Then, by Assumption \ref{Assumption: LPCA}, $\frac{1}{p}\bF_{\gr{0}, \subi}'\widehat{\bF}_{\gr{0},\subi}$
	is of full rank, and thus $\tilde{\bR}_{0, \subi}$ is invertible w.p.a. 1.
	Insert it into the projection matrix:
	\[
	\begin{split}
		\bP_{\widehat{\bF}_{\gr{0},\subi}}-\bP_{\bF_{\gr{0},\subi}}
		=&\frac{1}{p}\widehat{\bF}_{\gr{0},\subi}\widehat{\bF}_{\gr{0},\subi}'\\
		&-\frac{1}{p}\bF_{\gr{0},\subi}\tilde{\bR}_{0,\subi}\Big(\frac{1}{p}\tilde{\bR}_{0,\subi}'\bF_{\gr{0},\subi}'\bF_{\gr{0},\subi}\tilde{\bR}_{0,\subi}\Big)^{-1}\tilde{\bR}_{0,\subi}'\bF_{\gr{0},\subi}'.
	\end{split}
	\]
	By results in part (ii) and Assumption \ref{Assumption: LPCA}(a), 
	$\frac{1}{p}\|\widehat{\bF}_{\gr{0},\subi}-\bF_{\gr{0},\subi}\tilde{\bR}_{0,\subi}\|_{\mathtt{F}}^2\lesssim_\P \delta_{n}^{-2}+(\upsilon_{\bar\ttd_{i1},\subi})^4$ uniformly over $\subi$.
	Since $\frac{1}{p^\ddagger}\widehat{\bF}_{\gr{0},\subi}'\widehat{\bF}_{\gr{0},\subi}=\bI_{\ttd_{i0}}$, the matrix in the bracket is also invertible w.p.a.1 and thus the above expression is well defined. Using the fact that for any two invertible matrices $\bA$ and $\bB$, $\bA^{-1}-\bB^{-1}=\bA^{-1}(\bB-\bA)\bB^{-1}$, we can see that
	$\|\bP_{\widehat{\bF}_{\gr{0},\subi}}-\bP_{\bF_{\gr{0},\subi}}\|_{\mathtt{F}}^2\lesssim_\P \delta_{n}^{-2}+(\upsilon_{\bar\ttd_{i1},\subi})^4$
	uniformly over $\subi$.
\end{proof}
\bigskip

Now, we extend the results to higher-order eigenvalues and eigenvectors to finish the proof of Lemma \ref{lem: consistency eigenstructure}.
	The proof is divided into several steps.
	
	\textit{Step 1: Second-order eigenvalues}.
	Decompose $\bM_{\widehat{\bF}_{\gr{0},\subi}}\bX_{\subi}\bX_{\subi}'\bM_{\widehat{\bF}_{\gr{0},\subi}}$ the same way as in the proof of Lemma \ref{lem: eigenstructure 1st order} and  define $\bG_1, \bG_2, \cdots, \bG_4$ accordingly. 
	
	For $\bG_1$, write
	\[
	\begin{split}
		\bG_1=&\bM_{\widehat{\bF}_{\gr{0},\subi}}\bF_{\subi}\bLambda_{\subi}'\bLambda_{\subi}\bF_{\subi}'\bM_{\widehat{\bF}_{\gr{0},\subi}}\\
		=&(\bM_{\widehat{\bF}_{\gr{0},\subi}}-\bM_{\bF_{\gr{0},\subi}})\bF_{\subi}\bLambda_{\subi}'\bLambda_{\subi}\bF_{\subi}'\bM_{\widehat{\bF}_{\gr{0},\subi}}
		+\\
		&\bM_{\bF_{\gr{0},\subi}}\bF_{\subi}\bLambda_{\subi}'\bLambda_{\subi}\bF_{\subi}'(\bM_{\widehat{\bF}_{\gr{0},\subi}}-\bM_{\bF_{\gr{0},\subi}})+\\
		&\bM_{\bF_{\gr{0},\subi}}\bF_{\subi}\bLambda_{\subi}'\bLambda_{\subi}\bF_{\subi}'\bM_{\bF_{\gr{0},\subi}}
		=: \bG_{1,1}+\bG_{1,2}+\bG_{1,3}.
	\end{split}
	\]
	Note that the three terms are defined locally for each neighborhood $\mathcal{N}_i$ and this implicit dependence on $\subi$ is suppressed for simplicity. 
	By Assumption \ref{Assumption: LPCA}, it is immediate that 
	$s_j(\frac{1}{pK}\bG_{1,3})\asymp_\P (\upsilon_{\bar\ttd_{i1}, \subi})^2$ for all $1\leq i\leq n$ and $j=1, \ldots, \ttd_{i1}$. 
	Since $\underset{1\leq i\leq n}{\max}\frac{1}{\sqrt{pK}}\|\bM_{\bF_{\gr{0},\subi}}\bF_{\subi}\bLambda_{\subi}'\|\\
	\lesssim_\P \upsilon_{\bar\ttd_{i1}, \subi}$, using
	part (iii) of Lemma \ref{lem: eigenstructure 1st order}, 
	$\|\frac{1}{pK}\bG_{1,2}\|\lesssim_\P
	(\delta_n^{-1}+(\upsilon_{\bar\ttd_{i1},\subi})^2)\upsilon_{\bar\ttd_{i1},\subi}$ uniformly over $i$.
	For $\bG_{1,1}$, further decompose the projection matrix on the far right: $\bM_{\widehat{\bF}_{\gr{0},\subi}}=\bM_{\widehat{\bF}_{\gr{0},\subi}}-\bM_{\bF_{\gr{0},\subi}}+\bM_{\bF_{\gr{0},\subi}}$. By similar calculation, it can be shown that 
	$\|\frac{1}{pK}\bG_{1,1}\|\lesssim_\P
	(\delta_{n}^{-1}+(\upsilon_{\bar\ttd_{i1},\subi})^2)^2+(\delta_n^{-1}+(\upsilon_{\bar\ttd_{i1},\subi})^2)\upsilon_{\bar\ttd_{i1},\subi}$ uniformly over $i$.
	Therefore, $\bG_{1,1}$ is dominated by $\bG_{1,3}$ due to the rate condition that $\upsilon_{\bar\ttd_{i1},\subi}\delta_n\rightarrow\infty$.
	
	For $\bG_2$, the analysis is the same as that in the proof of Lemma \ref{lem: eigenstructure 1st order} (the projection operator  $\bM_{\widehat{\bF}_{\gr{0},\subi}}$ does not change the upper bound).

	For $\bG_3$ or $\bG_4$, note that 
	\[
	\begin{split}
		\frac{1}{pK}\bM_{\widehat{\bF}_{\gr{0},\subi}}\bF_{\subi}\bLambda_{\subi}'\bU_{\subi}'\bM_{\widehat{\bF}_{\gr{0},\subi}}
		=&\frac{1}{pK}\bM_{\bF_{\gr{0},\subi}}\bF_{\subi}\bLambda_{\subi}'\bU_{\subi}'\bM_{\widehat{\bF}_{\gr{0},\subi}}\\
		&+\frac{1}{pK}(\bM_{\widehat{\bF}_{\gr{0},\subi}}-\bM_{\bF_{\gr{0},\subi}})\bF_{\subi}\bLambda_{\subi}'\bU_{\subi}'\bM_{\widehat{\bF}_{\gr{0},\subi}}.
	\end{split}
	\]
	By the same truncation argument used before, the first term is $O_\P(\sqrt{\log (n\vee p)/K}\upsilon_{\bar\ttd_{i1},\subi})$ uniformly over $\subi$, and the second one is $O_\P((\delta_n^{-1}+(\upsilon_{\bar\ttd_{i1},\subi})^2)\sqrt{\log (n\vee p)/K})$. Then, the result for the second-order eigenvalues follows.
	
	\textit{Step 2: Second-order eigenvectors}. 
	The proof is similar to that of Lemma \ref{lem: eigenstructure 1st order}, but we need to rewrite  \eqref{eq: decomposition}:
	\begin{align*}
		&\bM_{\widehat{\bF}_{\gr{0},\subi}}\widehat{\bF}_{\gr{1},\subi}-
		\bM_{\widehat{\bF}_{\gr{0},\subi}}\bF_{\subi}\tilde{\bR}_{\gr{1},\subi}\\
		=\bigg\{&\frac{1}{pK}\bM_{\widehat{\bF}_{\gr{0},\subi}}\bF_{\subi}\bLambda_{\subi}'\bU_{\subi}'\widehat{\bF}_{\gr{1},\subi}+
		\frac{1}{pK}\bM_{\widehat{\bF}_{\gr{0},\subi}}\bU_{\subi}\bLambda_{\subi}\bF_{\subi}' \bM_{\widehat{\bF}_{\gr{0},\subi}}\widehat{\bF}_{\gr{1},\subi}+\nonumber\\
		&\frac{1}{pK}\bM_{\widehat{\bF}_{\gr{0},\subi}}\bF_{\subi}\bLambda_{\subi}'\bXi_{\subi}'\widehat{\bF}_{\gr{1},\subi}+
		\frac{1}{pK}\bM_{\widehat{\bF}_{\gr{0},\subi}}\bXi_{\subi}\bLambda_{\subi}\bF_{\subi}'\bM_{\widehat{\bF}_{\gr{0},\subi}}\widehat{\bF}_{\gr{1},\subi}+\nonumber\\
		&\frac{1}{pK}\bM_{\widehat{\bF}_{\gr{0},\subi}}\bXi_{\subi}\bU_{\subi}'\widehat{\bF}_{\gr{1},\subi}+
		\frac{1}{pK}\bM_{\widehat{\bF}_{\gr{0},\subi}}\bU_{\subi}\bXi_{\subi}'\widehat{\bF}_{\gr{1},\subi}+\nonumber\\
		&\frac{1}{pK}\bM_{\widehat{\bF}_{\gr{0},\subi}}\bXi_{\subi}\bXi_{\subi}'\widehat{\bF}_{\gr{1},\subi}+
		\frac{1}{pK}\bM_{\widehat{\bF}_{\gr{0},\subi}}\bU_{\subi}\bU_{\subi}'\widehat{\bF}_{\gr{1},\subi}
		\bigg\}\times \widehat{\bOmega}_{\mathcal{C}_1\mathcal{C}_1,\subi}^{-1},
	\end{align*}
	where $\widehat{\bOmega}_{\mathcal{C}_1\mathcal{C}_1,\subi}$ is a diagonal matrix that contains the next $\ttd_{i1}$ leading eigenvalues of $\frac{1}{pK}\bX_{\subi}\bX_{\subi}'$.
	Note that in part (iii) of Lemma \ref{lem: eigenstructure 1st order}, 
	$\underset{1\leq i\leq n}{\max}
	\|\bM_{\widehat{\bF}_{\gr{0},\subi}}-\bM_{\bF_{\gr{0},\subi}}\|_{\mathtt{F}}\lesssim_\P\delta_n^{-1}+
	(\upsilon_{\bar\ttd_{i1},\subi})^2$.
	Repeating the argument in Step 1 and Lemma \ref{lem: eigenstructure 1st order}, we have
	$$
	\max_{1\leq i\leq n}\frac{1}{\sqrt{p}}\|\bM_{\widehat{\bF}_{\gr{0},\subi}}\widehat{\bF}_{\gr{1},\subi}-\bM_{\bF_{ \subi}\tilde{\bR}_{\gr{0},\subi}}\bF_{\subi}\tilde{\bR}_{\gr{1},\subi}\|_{\mathtt{F}}\lesssim_\P 
	\delta_n^{-1}(\upsilon_{\bar\ttd_{i1},\subi})^{-1}+h_n^{2m}(\upsilon_{\bar\ttd_{i1},\subi})^{-2}
	$$
	and $\bM_{\bF_{\subi}\tilde{\bR}_{\gr{0},\subi}}\bF_{\subi}\tilde{\bR}_{\gr{1},\subi}=\bF_{\subi}\check{\bR}_{\gr{1},\subi}$ for some $\check{\bR}_{\subi}$.  
	Thus, the result for the second-order eigenvectors follows (the expression of $\check{\bR}_{\subi}$ will be given at the end of the proof).
	
	\textit{Step 3: Extension to higher-order terms}.
	The above calculation can be applied to even higher-order approximation as long as the rate condition $\delta_{n}^{-1}\upsilon_{\ttd_i,\subi}^{-1}=o(1)$ is satisfied. 
	For instance, consider the third-order approximation.	
	Define $\bar{\mathcal{C}}_{i1}=\mathcal{C}_{i0}\cup\mathcal{C}_{i1}$.
	To mimic the strategy before, the key is to analyze
	$
	\bM_{\widehat{\bF}_{\cdot\bar{\mathcal{C}}_{i1},\subi}}\bM_{\widehat{\bF}_{\gr{0},\subi}}\bF_{\cdot\bar{\mathcal{C}}_{i1},\subi}\bLambda_{\cdot\bar{\mathcal{C}}_{i1},\subi}'=
	\bM_{\widehat{\bF}_{\cdot\bar{\mathcal{C}}_{i1},\subi}}\bM_{\widehat{\bF}_{\gr{0},\subi}}\bF_{\gr{0},\subi}\bLambda_{\gr{0},\subi}'+
	\bM_{\widehat{\bF}_{\cdot\bar{\mathcal{C}}_{i1},\subi}}\bM_{\widehat{\bF}_{\gr{0},\subi}}\bF_{\gr{1}\subi}\bLambda_{\gr{1},\subi}'
	=:\mathrm{I}+\mathrm{II}.
	$
	By a similar argument used in the previous step, $(pK)^{-1/2}\|\mathrm{II}\|\lesssim_\P\upsilon_{\bar\ttd_{i1},\subi}(\delta_{n}^{-1}/\upsilon_{\bar\ttd_{i1},\subi}+\upsilon_{\bar\ttd_{i2},\subi}^2/(\upsilon_{\bar\ttd_{i1},\subi})^2)=o_\P(\upsilon_{\bar\ttd_{i2},\subi})$ uniformly over $i$. 
	For $\mathrm{I}$,
	\[
	\begin{split}
		-\mathrm{I}=&\bM_{\widehat{\bF}_{\cdot\bar{\mathcal{C}}_{i1},\subi}}(\bP_{\widehat{\bF}_{\gr{0},\subi}}-\bP_{\bF_{\gr{0},\subi}})\bF_{\gr{0},\subi}\bLambda_{\gr{0},\subi}'\\
		=&\bM_{\widehat{\bF}_{\cdot\bar{\mathcal{C}}_{i1},\subi}}\Big\{
		\frac{1}{p}(\widehat{\bF}_{\gr{0},\subi}-\bF_{\gr{0},\subi}\tilde{\bR}_{0,\subi})\times\widehat{\bF}_{\gr{0},\subi}'\\
		&+\frac{1}{p}\bF_{\gr{0},\subi}\tilde{\bR}_{0,\subi}\Big(\widehat{\bF}_{\gr{0},\subi}'-
		\Big(\frac{1}{p}\tilde{\bR}_{0,\subi}'\bF_{\gr{0}, \subi}'\bF_{\gr{0}, \subi}\tilde{\bR}_{0,\subi}\Big)^{-1}\bF_{\gr{0}, \subi}'\Big)\Big\}\bF_{\gr{0},\subi}\bLambda_{\gr{0},\subi}'.
	\end{split}
	\]
	By the rate condition, the results in part (iii) of Lemma \ref{lem: eigenstructure 1st order} and step 2 of this proof, the second term divided by $\sqrt{pK}$ is $o_\P(\upsilon_{\bar\ttd_{i2},\subi})$ uniformly over $i$ in terms of $\|\cdot\|$-norm.
	For the first term on the right-hand side, plug in the expansion for $\widehat{\bF}_{\gr{0},\subi}-\bF_{\gr{0}, \subi}\tilde{\bR}_{0,\subi}$. By consistency of $\bM_{\widehat{\bF}_{\cdot\bar{\mathcal{C}}_1,\subi}}$, 
	$$
	\max_{1\leq i\leq n}\Big\|\frac{1}{p^2K}
	\bM_{\widehat{\bF}_{\cdot\bar{\mathcal{C}}_{i1},\subi}}
	\bF_{\gr{1},\subi}\bLambda_{\gr{1},\subi}'\bLambda_{\gr{1},\subi}\bF_{\gr{1},\subi}\widehat{\bF}_{\gr{0},\subi}\widehat{\bF}_{\gr{0},\subi}'
	\Big\|=o_\P(\upsilon_{\bar\ttd_{i2},\subi}).
	$$
	Other terms in the expansion are at most $O_\P(\delta_n^{-1})=o_\P(\upsilon_{\bar\ttd_{i2},\subi})$ uniformly over $i$ in terms of $\|\cdot\|$-norm. Then, we have $\underset{1\leq i\leq n}{\max}\|\frac{1}{\sqrt{pK}}\bM_{\widehat{\bF}_{\cdot\bar{\mathcal{C}}_{i1},\subi}}\bM_{\widehat{\bF}_{\gr{0},\subi}}\bF_{\cdot\bar{\mathcal{C}}_{i1},\subi}\bLambda_{\cdot\bar{\mathcal{C}}_{i1},\subi}'\|=o_\P(\upsilon_{\bar\ttd_{i2},\subi})$.
	With this preparation, the remainder of the proof for higher-order approximations is the same as that used before.
	
	\textit{Step 4:} Finally, a typical $j$th column of the re-defined rotation matrix $\check{\bR}_{\subi}$ is given by 
	$\check{\bR}_{\cdot j, \subi}=
	\tilde{\bR}_{\cdot j, \subi}-\tilde{\bR}_{1:(j-1), \subi}(\tilde{\bR}_{1:(j-1), \subi}\bF_{\subi}'\bF_{\subi}\tilde{\bR}_{1:(j-1), \subi})^{-1}\tilde{\bR}_{1:(j-1), \subi}\bF_{\subi}'\bF_{\subi}\tilde{\bR}_{\cdot j,\subi}$,
	where $\tilde{\bR}_{1:(j-1), \subi}$ is the leading $(j-1)$ columns of $\tilde{\bR}_{\subi}$. Therefore,
	$\bF_{\subi}\check{\bR}_{\subi}$ is a columnwise orthogonalized version of $\bF_{\subi}\tilde{\bR}_{\subi}$.

\subsection{Proofs for Section \ref{SA-sec: main results}}

\subsubsection{Proof of Lemma \ref{SA-lem: slope of covariates}}
	Let $p^\ddagger=|\mathcal{R}^\ddagger|$. Rewrite Equation \eqref{SA-eq: general model} as
	\[
	\begin{split}
	x_{it}=\sum_{\ell=1}^{q}\hbar_{t,\ell}(\bvrho_{i,\ell})\vartheta_\ell+
	\sum_{\ell=1}^{q}e_{it, \ell}\vartheta_\ell
	+\eta_t(\balpha_i)+u_{it}
	=\hslash_{t}(\bvrho_i)+
	\sum_{\ell=1}^{q}e_{it,\ell}\vartheta_\ell+u_{it},
	\end{split}
	\]
	where $\hslash_{t}(\bvrho_{i})=
	\eta_t(\balpha_i)+\sum_{\ell=1}^{q}\hbar_{t,\ell}(\bvrho_{i,\ell})
	\vartheta_\ell$ and $\bvrho_{i}$ is a vector collecting all distinct variables among $\balpha_i,\bvrho_{i,1},\cdots, \bvrho_{i,q}$. Note that $\balpha_i$ is included in $\bvrho_i$ as a subvector. 
	
	We first prepare some notation.  Define  $\hslash_{it}:=\hslash_t(\bvrho_i)$, and stack all $\hbar_{it}$'s with $t\in\mathcal{R}^\ddagger$ in a $p^\ddagger$-vector $\bm{\hslash}_{i}$. Similarly, for each $\ell=1,\ldots, q$, define $\hbar_{it,\ell}:=\hbar_{t,\ell}(\bvrho_{i,\ell})$ and a $p^\ddagger$-vector $\bm{\hbar}_{i,\ell}$ with typical elements $\hbar_{it,\ell}$ for $t\in\mathcal{R}^\ddagger$, and let $\be_{i,\ell}$ be a $p^\ddagger$-vector with typical elements $e_{it,\ell}$ for $t\in\mathcal{R}^\ddagger$ and $\be_i=(\be_{i,1}, \cdots, \be_{i,q})'$. 
	Given the estimation procedure described in Section \ref{subsec: extensions}, 
	we let $\widehat{\bm{\hbar}}_{i,\ell}$ and  $\widehat{\bm{\hslash}}_i$ be the 
	``estimators'' of $\bm{\hbar}_{i,\ell}$ and $\bm{\hslash}_i$ obtained in Step (b) and Step (c) respectively, and recall
	that $\widehat{\be}_i$ is the estimation residual from Step  (b).
	Then write
	\[
	\begin{split}
	\widehat{\bvth}-\bvth=
	&\Big(\frac{1}{np^\ddagger}\sum_{i=1}^{n}\widehat{\be}_i\widehat{\be}_i'\Big)^{-1}\times
	\bigg\{\Big(\frac{1}{np^\ddagger}\sum_{i=1}^{n}
	\widehat{\be}_i\bu_i\Big)+
	\Big(\frac{1}{np^\ddagger}\sum_{i=1}^{n}\widehat{\be}_i(\be_i-\widehat{\be}_i)'\bvth\Big)+\\
	&\hspace{9.5em}\Big(\frac{1}{np^\ddagger}\sum_{i=1}^{n}\widehat{\be}_i(\bm{\hslash}_{i}-\widehat{\bm{\hslash}}_{i})\Big)\bigg\}\\
	=&\Big(\frac{1}{np^\ddagger}\sum_{i=1}^{n}\widehat{\be}_i\widehat{\be}_i'\Big)^{-1}\times(I_1+I_2+I_3).
	\end{split}
	\]
	
	Now, first notice that
	\begin{align*}
	\frac{1}{np^\ddagger}\sum_{i=1}^{n}\widehat{\be}_i\widehat{\be}_i'=
	&\frac{1}{np^\ddagger}\sum_{i=1}^{n}\be_i\be_i'+
	\frac{1}{np^\ddagger}\sum_{i=1}^{n}(\widehat{\be}_i-\be_i)(\widehat{\be}_i-\be_i)'+\\
	&\frac{1}{np^\ddagger}\sum_{i=1}^{n}(\widehat{\be}_i-\be_i)\be_i'+
	\frac{1}{np^\ddagger}\sum_{i=1}^{n}\be_i(\widehat{\be}_i-\be_i)'.
	\end{align*}
	By Assumption \ref{SA-Assumption: high-rank covariates}, the first term is bounded away from zero w.p.a. 1.  
	Note that for each $\ell\in[q]$, $\widehat{\be}_{i,\ell}-\be_{i,\ell}=
	\bm{\hbar}_{i,\ell}-\widehat{\bm{\hbar}}_{i,\ell}$.
	Under Assumptions \ref{SA-Assumption: high-rank covariates}--\ref{SA-Assumption: local approximation}, 
	the conditions of Corollary \ref{coro: consistency of latent mean} in the main paper are satisfied and hence 
	$\max_{1\leq i\leq n}
	\|\widehat{\bm{\hbar}}_i-\bm{\hbar}_i\|_{\max}=o_\P(1)$.
	Therefore, the last three terms are $o_\P(1)$.
	
	Next, consider $I_2$. For any $1\leq \ell, \ell'\leq q$, by Corollary \ref{coro: consistency of latent mean} in the main paper,
		\[
		\begin{split}
		&\frac{1}{np^\ddagger}\sum_{i=1}^{n}\sum_{t\in\mathcal{R}^\ddagger}
		\widehat{e}_{it,\ell}(e_{it,\ell'}-\widehat{e}_{it,\ell'})\\
		=&\frac{1}{np^\ddagger}\sum_{i=1}^{n}\sum_{t\in\mathcal{R}^\ddagger}
		e_{it,\ell}(\widehat{\hbar}_{it,\ell'}-\hbar_{it,\ell'})+
		\frac{1}{np^\ddagger}\sum_{i=1}^{n}\sum_{t\in\mathcal{R}^\ddagger}
		(\hbar_{it,\ell}-\widehat{\hbar}_{it,\ell})(\widehat{\hbar}_{it,\ell'}-\hbar_{it,\ell'})\\
		=& I_{2,1}+O_\P(\delta_n^{-2}+h_{n,\varrho}^{2m}).
		\end{split}
		\]
	For $I_{2,1}$, by construction, we can write the $\widehat{\hbar}_{it,\ell'}-\hbar_{it,\ell'}=
	-\xi_{it,\ell',\subi}+
	\widehat{\bff}_{t,\ell',\subi}'\widehat{\blambda}_{i,\ell',\subi}-
	\bff_{t,\ell',\subi}'\blambda_{i,\ell',\subi}$ where 
	$\xi_{it,\ell',\subi}$ is the approximation error for $\hbar_{it,\ell'}$, and 
	$\widehat{\bff}_{t,\ell',\subi}$ and $\widehat{\blambda}_{i,\ell',\subi}$ denote the factors corresponding to ``feature $t$'' and factor loadings corresponding to ``unit $i$'' extracted from $\{\bw_{i,\ell'}: 1\leq i\leq n\}$. Also, we will use $\bR_{\ell',\subi}$ and $\widehat{\boldsymbol{\Omega}}_{\ell',\subi}$ to denote the rotation matrix and the matrix of eigenvalues from the local PCA for the $\ell'$th regressor $\bw_{i,\ell'}$ (understood the same way as in Equation \eqref{SA-eq: decomp of factors}). 
	It is easy to see that 
	$\frac{1}{np^\ddagger}\sum_{i=1}^{n}\sum_{t\in\mathcal{R}^\ddagger}\xi_{it,\ell',\subi}e_{it,\ell}\lesssim_\P h_{n,\varrho}^{m}p^{-1/2}$. 
	Moreover,
	\[
	\begin{split}
	&\frac{1}{np^\ddagger}\sum_{i=1}^{n}\sum_{t\in\mathcal{R}^\ddagger}
	(\widehat{\bff}_{t,\ell',\subi}'\widehat{\blambda}_{i,\ell',\subi}-
	\bff_{t,\ell',\subi}'\blambda_{i,\ell',\subi})e_{it,\ell}\\
	=&\frac{1}{np^\ddagger}\sum_{i=1}^{n}\sum_{t\in\mathcal{R}^\ddagger}
	(\widehat{\bff}_{t,\ell',\subi}'-\bff_{t,\ell',\subi}'(\bR_{\ell',\subi}')^{-1})\widehat{\blambda}_{i,\ell',\subi}e_{it,\ell}+\\
	&\frac{1}{np^\ddagger}\sum_{i=1}^{n}\sum_{t\in\mathcal{R}^\ddagger}
	\bff_{t,\ell',\subi}'(\bR_{\ell',\subi}')^{-1}(\widehat{\blambda}_{i,\ell',\subi}-
	\bR_{\ell',\subi}'\blambda_{i,\ell',\subi})e_{it,\ell}
	=:I_{2,1,1}+I_{2,1,2}.
	\end{split}
	\]
	
	For $I_{2,1,1}$, plug in the expansion of the estimated factors as in Equation \eqref{SA-eq: decomp of factors} in the main paper:
	\[
	\begin{split}
	&\frac{1}{p^\ddagger}\sum_{t\in\mathcal{R}^\ddagger}(\widehat{\bff}_{t,\ell',\subi}'-\bff_{t,\ell',\subi}'(\bR_{\ell',\subi}')^{-1})e_{it,\ell}\widehat{\blambda}_{i,\ell',\subi}\\
	=&\Big\{\frac{1}{Kp^\ddagger}\sum_{t\in\mathcal{R}^\ddagger}\sum_{k=1}^{K}e_{it,\ell}\bff_{t,\ell',\subi}'(\bR_{\ell',\subi}')^{-1}(\bR_{\ell',\subi}'\blambda_{j_k(i),\ell',\subi}-\widehat{\blambda}_{j_k(i),\ell',\subi})\widehat{\blambda}_{j_k(i),\ell',\subi}'\\
	&+\frac{1}{Kp^\ddagger}\sum_{t\in\mathcal{R}^\ddagger}\sum_{k=1}^{K}e_{it,\ell}e_{j_k(i)t,\ell'}
	\widehat{\blambda}_{j_k(i),\ell',\subi}'+
	\frac{1}{Kp^\ddagger}\sum_{t\in\mathcal{R}^\ddagger}\sum_{k=1}^{K}e_{it,\ell}\xi_{j_k(i)t,\ell',\subi}\widehat{\blambda}_{j_k(i),\ell',\subi}'\Big\}\times\widehat{\boldsymbol{\Omega}}_{\ell',\subi}^{-1}\widehat{\blambda}_{i,\ell',\subi}.
	\end{split}
	\]
	By the argument in the proof of Theorem \ref{thm: uniform convergence of factors}, $\frac{1}{Kp^\ddagger}\sum_{t\in\mathcal{R}^\ddagger}\sum_{k=1}^{K}e_{it,\ell}e_{j_k(i)t,\ell'}\widehat{\blambda}_{j_k(i),\ell',\subi}'\widehat{\bOmega}_{\ell',\subi}^{-1/2}\lesssim_\P\delta_n^{-1}$. 
	By Assumptions \ref{SA-Assumption: regularities} and \ref{SA-Assumption: local approximation}, $\frac{1}{p^\ddagger}\sum_{t\in\mathcal{R}^\ddagger}e_{it,\ell}\xi_{j_k(i)t,\ell',\subi}\lesssim_\P h_{n,\varrho}^{m}\delta_n^{-1}$ uniformly over $k$ and $i$. 
	By Theorem  \ref{thm: uniform convergence of factors} and the fact that  
	$\frac{1}{p^\ddagger}\sum_{t\in\mathcal{R}^\ddagger}\bff_{t,\ell',\subi}'e_{it,\ell}
	\lesssim_\P \delta_n^{-1}$ uniformly over $k$ and $i$, the first term in $I_{2,1,1}$ is of smaller order.
	Then, it follows that $I_{2,1,1}=O_\P(\delta_n^{-1}+h_{n,\varrho}^{m}\delta_n^{-1})$. 
	Moreover, by Theorem  \ref{thm: uniform convergence of factors}, 
	$I_{2,1,2}=O_\P(\delta_n^{-1}(\delta_n^{-1}+h_{n,\varrho}^{m}))$.
	$I_3$ can be treated similarly. 
	
	Finally, for $I_1$,
	$\frac{1}{np^\ddagger}\sum_{i=1}^{n}
	\widehat{\be}_i\bu_i=
	\frac{1}{np^\ddagger}\sum_{i=1}^{n}
	\be_i\bu_i+\frac{1}{np^\ddagger}\sum_{i=1}^{n}
	(\widehat{\be}_i-\be_i)\bu_i$. 
	Note that $\E[\bu_i|\bw_i]=0$ and $\E[\bu_i|\mathcal{F}]=0$ imply that $\bu_i$ is uncorrelated with $\be_i$.  
	Then, by Assumption \ref{SA-Assumption: regularities}, the first term is $O_\P(1/\sqrt{np})$. The second term is mean zero and of smaller order due to the consistency of $\widehat{\be}_i$. Then, the proof is complete.

\subsubsection{Proof of Theorem \ref{SA-thm: relevant FE}}
	By construction, we use the subsample $\mathcal{R}^\dagger$ for initial matching on $\bx_i$ and $\bw_{i,\ell}$'s, and then apply local PCA to the subsample $\mathcal{R}^\ddagger$ to obtain  $\widehat{\bvth}$. Now we consider the final step of getting the local factors and factor loadings of interest.
	
	By Assumption \ref{SA-Assumption: indirect matching} and Theorem \ref{thm: IMD} given in the main paper, we can immediately obtain the following bound on the matching discrepancy: 
	$$\max_{1\leq i\leq n}
	\max_{1\leq k\leq K}
	\|\balpha_i-\balpha_{j_k(i)}\|\lesssim_\P
	(K/n)^{\uvarsig/(\lvarsig r)}
	+a_n^{1/\lvarsig}.$$
	
	Next,  recall that the local PCA is conducted on the subsample $\mathcal{R}^\wr$ to ensure the factor components and noises are uncorrelated. 
	Let $p^\wr=|\mathcal{R}^\wr|$. 
	Apply the results of Theorem  \ref{thm: uniform convergence of factors} in the main paper with minor modification. Specifically, we have
	\[
	\widehat{\bLambda}_{\subi}-\bLambda_{\subi}\bR_{\subi}=
	\frac{1}{p^\wr}\bXi_{\subi}'\widehat{\bF}_{\subi}+
	\frac{1}{p^\wr}\bU_{\subi}'\widehat{\bF}_{\subi}+
	\frac{1}{p^\wr}(\bvth-\widehat{\bvth})'\tilde{\bW}_{\subi}'\widehat{\bF}_{\subi}
	\]
	where $\tilde{\bW}_{\subi}$ is a $p^\wr\times K\times q$ matrix with $\ell$th sheet given by $(\bw_{\mathcal{R}^\wr,j_1(i),\ell}, \cdots, \bw_{\mathcal{R}^\wr,j_K(i),\ell})$ associated with the $q$-dimensional coefficient $\bvth$. Here $\bw_{\mathcal{R}^\wr,j_k(i),\ell}$ is the subvector of $\bw_{j_k(i),\ell}$ with the indices in $\mathcal{R}^\wr$. Note that the rate condition $\delta_{n}h_{n,\varrho}^{2m}\lesssim 1$ implies that $h_{n,\varrho}^{2m}=o(\upsilon_{\ttd_i^{\textsf{M}},\subi})$ for $\bM=\bH_{\subi}$. Thus, additional approximation error in the final local PCA step that arises from $\tilde\bW_i(\widehat{\bvth}-\bvth)$ is still dominated by the last factor extracted.  Then, the first two terms in the above decomposition can be treated exactly the same way as in the proof of Theorem  \ref{thm: uniform convergence of factors}, and the third term is trivially $O_\P(\|\bvth-\widehat{\bvth}\|)$. Then, the desired result for the estimated loadings follows from Lemma \ref{SA-lem: slope of covariates}. The result for the estimated factors follows by the same argument as in the proof of Theorem \ref{thm: uniform convergence of factors}.

%%%%%%%%%%%%%%%%%%%%%%%%%%%%%%%%%%%%%
\section{Additional Simulation Results}\label{SA-sec: simulation}

In the following we present the additional simulation results for the three models described in the main paper. 

Table \ref{table:simul, p=500} presents results for the case $p=500$. We still use the first half of rows for $K$-NN matching and the second half for local PCA. We can see the main findings are similar to those for the case $p=1\,000$.
The improvement of local PCA over global PCA is not pronounced in Model 3, since in this binary model the noise is large relative to the ``signal'' (nonlinearity of the latent surface), especially when $p$ is small.

Next, in Table \ref{table:simul, p=500, 0.8knn} we consider the same scenario as in Table \ref{table:simul, p=500} but use more features (80\% of rows) for $K$-NN matching and fewer features (20\%) for local PCA. Thus, PCA is conducted based on a submatrix of $\bX$ with $p$ and $K$ more balanced. We can see the performance of local PCA does not change much in Models 2 and 3. By contrast, the prediction errors for missing entries in Model 1 significantly increase. This can be explained by the large nonlinearity of this model, where using smaller number of features for PCA greatly restricts our ability to extract weaker factors that capture higher-order nonlinearity of the latent functions.

\FloatBarrier
\begin{table}[h]
	\centering
	\scriptsize
	\caption{Simulation Results, $n=1\,000$, $p=500$, $50\%$ for KNN, $2\,000$ replications}
	\label{table:simul, p=500}
	\resizebox{.65\textwidth}{1.2\height}{\footnotesize \input{input/Table_MainPaper2.txt}}
	\flushleft\footnotesize{\textbf{Notes}:
		MAE = maximum absolute error; $q_\alpha$:  $\alpha$-quantile of $\{\alpha_i: 1\leq i\leq n\}$.
	}\newline
\end{table}
\FloatBarrier

\FloatBarrier
\begin{table}[h]
	\centering
	\scriptsize
	\caption{Simulation Results, $n=1\,000$, $p=500$, $80\%$ for KNN, $2\,000$ replications}
	\label{table:simul, p=500, 0.8knn}
	\resizebox{.65\textwidth}{1.2\height}{\footnotesize \input{input/Table_MainPaper4.txt}}
	\flushleft\footnotesize{\textbf{Notes}:
		MAE = maximum absolute error; $q_\alpha$:  $\alpha$-quantile of $\{\alpha_i: 1\leq i\leq n\}$.
	}\newline
\end{table}
\FloatBarrier

\bibliography{Feng_2023_NonlinearFactorModel--Bibliography}
\bibliographystyle{econometrica}

\makeatletter\@input{xx.tex}\makeatother

\end{document}
